# Supplementary material for: RadOncGym: An Agent-Based Framework for Radiotherapy Dose-Mimicking Optimization
Source: arXiv:2611.33821 source file (2026-11-25)
Supplement: Supplementary file 1 [file agent_behavior.tex]

\section{Agent-Loop and Weight-Update Details}
\label{supp:agent_behavior}

\begin{figure}[!t]
    \centering
    \includegraphics[width=0.62\columnwidth]
    {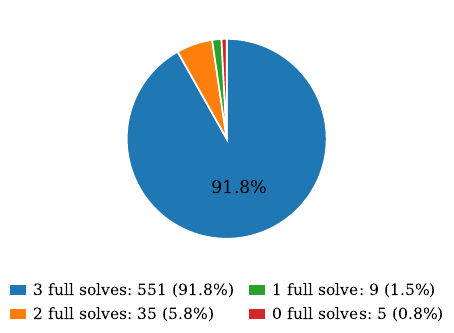}

    {\small (a) Successful full solves}

    \smallskip
    \includegraphics[width=0.82\columnwidth]
    {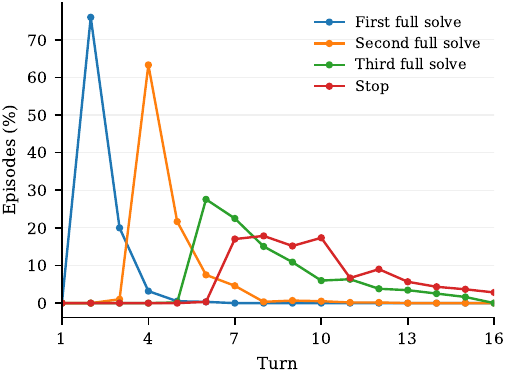}

    {\small (b) Full-solve and stopping-turn distributions}

    \caption{\textbf{Agent-loop behavior for GPT-5.6 Sol with criterion-response contrast memory and the candidate-critic role.} (a) Successful full solves per context. (b) Context frequency by turn for the first, second, and third successful full solves and the explicit stop.}
    \label{fig:loop_behavior}
\end{figure}

\subsection{Full-Solve Timing and Stage-Wise Gains}

\begin{table}[!t]
\centering
\scriptsize
\setlength{\tabcolsep}{2.7pt}
\textbf{(a) Episode-level use}\par\smallskip
\begin{tabular*}{\columnwidth}{@{\extracolsep{\fill}}lrrrr@{}}
\toprule
Quantity & $N$ & Mean & Median & Range \\
\midrule
Turns used & 600 & 9.92 & 9 & 6--16 \\
Successful full solves & 600 & 2.89 & 3 & 0--3 \\
Stop turn & 599 & 9.91 & 9 & 6--16 \\
\bottomrule
\end{tabular*}

\medskip
\textbf{(b) Timing and incumbent quality by solve stage}\par\smallskip
\begin{tabular*}{\columnwidth}{@{\extracolsep{\fill}}lrrrrrr@{}}
\toprule
Stage & $N$ reaching & \multicolumn{2}{c}{Turn} & $\Delta$Clin & $\Delta$DVH & $\Delta$Dose \\
\cmidrule(lr){3-4}
 & & Mean & Median [range] & & & \\
\midrule
Solve 1 & 595 & 2.29 & 2 [2--6] & 0.329 & 0.347 & 0.192 \\
Solve 2 & 586 & 4.60 & 4 [3--12] & 0.541 & 0.573 & 0.232 \\
Solve 3 & 551 & 8.23 & 7 [5--15] & 0.613 & 0.599 & 0.220 \\
\bottomrule
\end{tabular*}
\caption{\textbf{Episode timing and staged performance for the representative GPT-5.6 Sol agent.} Improvements are measured against the all-ones initialization. The two panels use different denominators: turn statistics are conditional on the $N$ contexts that reach a stage, whereas the endpoint means are over all 600 contexts, carrying the previous incumbent forward (or the all-ones fallback) for contexts that have not reached it. The final row therefore reproduces the 600-context values reported in the main paper. DVH and dose scores are computed post hoc. One context reaches the 16-turn horizon without an explicit stop. Selection
minimizes clinical-criterion violation only, so the post-hoc DVH and dose scores
need not improve monotonically across stages; dose-score improvement falls from $0.232$ to
$0.220$~Gy between solve 2 and solve 3.}
\label{tab:supp_solve_timing_stage}
\end{table}

Figure~\ref{fig:loop_behavior} and Table~\ref{tab:supp_solve_timing_stage} summarize how the agent spends its solve budget. The first solve occurs on turn 2 in 452 of 595 contexts, and the second occurs on turn 4 in 371 of 586 contexts. The third solve most commonly occurs on turns 6, 7, and 8 (152, 124, and 83 contexts). The successful-solve-count distribution is 5, 9, 35, and 551 contexts with zero, one, two, and three successful solves, respectively. Counts in this section are successful solves rather than requests: the campaign issues 1,765 full-solve requests, of which 33 time out, leaving 1,732 successful solves. Those timeouts fall in 21 contexts, 16 of which still yield a valid selected plan; Table~\ref{tab:supp_campaign} gives the full breakdown.

The first solve captures approximately 54\% of the final clinical-criterion gain and the second brings the carried-forward incumbent to approximately 88\%. A new candidate replaces the clinical incumbent in 77.1\% of contexts reaching the second solve and 65.5\% of contexts reaching the third.

\subsection{Per-Control Weight Movement}

Table~\ref{tab:supp_weight_movement} reports how the 12 weights move during an episode. A movement is counted when the relative change exceeds 5\%. Step movement compares consecutive accepted weight proposals; turn-1 and final movement compare against the all-ones initialization.

\begin{table*}[!t]
\centering
\begin{minipage}[t]{0.495\textwidth}
\centering
\scriptsize
\setlength{\tabcolsep}{1.5pt}
\textbf{(a) Per-control proposal and final movement}\par\smallskip
\begin{tabular*}{\linewidth}{@{\extracolsep{\fill}}lrrrrrr@{}}
\toprule
Control & Ever & T1 & Step & Factor & Up & Down \\
\midrule
PTV56 & 100.0\% & 100.0\% & 41.3\% & 1.19$\times$ & 69.2\% & 18.8\% \\
PTV63 & 100.0\% & 99.0\% & 22.4\% & 1.14$\times$ & 32.5\% & 56.5\% \\
PTV70 & 100.0\% & 99.7\% & 32.0\% & 1.10$\times$ & 96.2\% & 0.8\% \\
Brainstem & 99.5\% & 64.3\% & 33.2\% & 1.21$\times$ & 2.3\% & 88.3\% \\
Spinal cord & 99.3\% & 70.0\% & 35.2\% & 1.20$\times$ & 11.2\% & 74.2\% \\
Mandible & 99.5\% & 87.0\% & 31.2\% & 1.16$\times$ & 12.3\% & 74.0\% \\
Right parotid & 99.8\% & 90.3\% & 43.1\% & 1.22$\times$ & 65.7\% & 26.0\% \\
Left parotid & 99.8\% & 92.8\% & 40.4\% & 1.22$\times$ & 67.3\% & 26.2\% \\
Esophagus & 99.8\% & 89.5\% & 19.3\% & 1.14$\times$ & 5.2\% & 89.8\% \\
Larynx & 99.8\% & 94.7\% & 28.4\% & 1.18$\times$ & 24.5\% & 67.0\% \\
Ring falloff & 100.0\% & 97.7\% & 47.3\% & 1.28$\times$ & 25.2\% & 65.0\% \\
Posterior neck & 97.3\% & 19.3\% & 41.5\% & 1.23$\times$ & 13.8\% & 74.2\% \\
\bottomrule
\end{tabular*}
\end{minipage}\hfill
\begin{minipage}[t]{0.485\textwidth}
\centering
\scriptsize
\setlength{\tabcolsep}{2.4pt}
\textbf{(b) Movement frequency by accepted proposal index}\par\smallskip
\begin{tabular*}{\linewidth}{@{\extracolsep{\fill}}rrrrrr@{}}
\toprule
Proposal index & $N$ & Target & Serial & Mean-dose & Shaping \\
\midrule
1 & 600 & 99.6\% & 73.8\% & 91.8\% & 58.5\% \\
2 & 600 & 23.9\% & 18.7\% & 20.7\% & 20.5\% \\
3 & 600 & 48.8\% & 59.1\% & 57.3\% & 68.6\% \\
4 & 600 & 19.8\% & 20.6\% & 21.5\% & 30.4\% \\
5 & 600 & 39.3\% & 46.9\% & 37.1\% & 67.1\% \\
6 & 598 & 29.8\% & 32.4\% & 30.2\% & 46.4\% \\
7 & 496 & 32.3\% & 28.6\% & 30.1\% & 44.0\% \\
8 & 389 & 31.4\% & 32.0\% & 32.4\% & 45.5\% \\
9 & 298 & 32.3\% & 27.7\% & 33.2\% & 37.1\% \\
10 & 194 & 30.1\% & 28.0\% & 32.1\% & 36.9\% \\
11 & 154 & 31.8\% & 29.4\% & 33.3\% & 38.6\% \\
12 & 100 & 30.7\% & 30.7\% & 31.5\% & 36.0\% \\
13 & 66 & 28.8\% & 28.8\% & 34.1\% & 37.1\% \\
14 & 40 & 22.5\% & 28.3\% & 30.0\% & 38.7\% \\
15 & 18 & 9.3\% & 27.8\% & 26.4\% & 19.4\% \\
16 & 1 & 0.0\% & 0.0\% & 25.0\% & 0.0\% \\
\bottomrule
\end{tabular*}
\end{minipage}
\caption{\textbf{Planning-objective weight-update behavior for the representative GPT-5.6 Sol agent.} A movement is a relative change greater than 5\%. In (a), ``Ever,'' ``T1,'' and ``Step'' are proposal-movement frequencies; ``Factor'' is the typical multiplicative change across consecutive accepted proposals; and ``Up'' and ``Down'' give the fraction of contexts whose final proposal weight ends more than 5\% above or below the all-ones initialization. In (b), $N$ is the number of episodes reaching each proposal index and the remaining entries are family-level movement percentages. The four families are target coverage (PTV56, PTV63, PTV70), serial-OAR sparing (brainstem, spinal cord, mandible), mean-dose OAR sparing (both parotids, esophagus, larynx), and shaping (ring falloff, posterior neck); the same grouping and naming are used in Table~\ref{tab:supp_backbone_weights}. The stop action contains no weight vector and is excluded.}
\label{tab:supp_weight_movement}
\end{table*}

\subsection{Cross-Backbone Behavioral Comparison}

The three backbones share the same environment, memory mechanism, role
structure, turn horizon, and full-solve budget, so differences in how they act
reflect differences among the end-to-end model deployments under a common
RadOncGym protocol rather than differences in the protocol itself. The three
routes differ in provider, client, and default reasoning configuration as
described in Section~\ref{supp:reproducibility}, so these rows are not
controlled comparisons of model identity alone.
Table~\ref{tab:supp_backbone_timing} reports timing and termination and
Table~\ref{tab:supp_backbone_weights} reports weight-update behavior. Values
come from the 600 episode records of each campaign.

\begin{table*}[!t]
\centering
\small
\setlength{\tabcolsep}{4pt}
\renewcommand{\arraystretch}{1.08}
\textbf{(a) Turns, solve timing, and stopping (mean / median, with $N$ where conditional)}\par\smallskip
\begin{tabular*}{\textwidth}{@{\extracolsep{\fill}}lccccc@{}}
\toprule
Backbone & Turns used & Successful solves & First solve turn & Second solve turn & Third solve turn \\
\midrule
GPT-5.6 Sol     & 9.92 / 9   & 2.89 / 3 & 2.29 / 2 (595) & 4.60 / 4 (586) & 8.23 / 7 (551) \\
Claude Sonnet 5 & 10.47 / 10 & 2.93 / 3 & 1.85 / 2 (596) & 3.62 / 3 (593) & 6.63 / 6 (568) \\
Qwen3.6-27B     & 13.61 / 15 & 2.82 / 3 & 3.65 / 3 (580) & 5.70 / 5 (566) & 7.69 / 8 (544) \\
\bottomrule
\end{tabular*}

\medskip
\textbf{(b) Episode-level solve use and termination}\par\smallskip
\setlength{\tabcolsep}{4pt}
\begin{tabular*}{\textwidth}{@{\extracolsep{\fill}}lcccccc@{}}
\toprule
Backbone & 0 solves & 1 solve & 2 solves & 3 solves & Explicit stop & Reached horizon \\
\midrule
GPT-5.6 Sol     & 0.8\% (5)  & 1.5\% (9)  & 5.8\% (35) & 91.8\% (551) & 99.8\% (599) & 0.2\% (1)    \\
Claude Sonnet 5 & 0.7\% (4)  & 0.5\% (3)  & 4.2\% (25) & 94.7\% (568) & 83.2\% (499) & 16.8\% (101) \\
Qwen3.6-27B     & 3.3\% (20) & 2.3\% (14) & 3.7\% (22) & 90.7\% (544) & 64.7\% (388) & 35.3\% (212) \\
\bottomrule
\end{tabular*}
\caption{\textbf{Turn, solve-timing, and termination behavior of the three backbones.} All rows use criterion-response contrast memory, the candidate-critic role, a 16-turn horizon, and at most three full solves on the same 600 contexts. Solve-turn statistics are conditional on episodes that reached that solve, with $N$ in parentheses. Explicit-stop percentages count episodes that emitted a stop action; the remainder reached the horizon.}
\label{tab:supp_backbone_timing}
\end{table*}

All three backbones use the budget: each completes three successful full solves in more
than 90\% of contexts, so the endpoint gap is not explained by refusal to
escalate. The differences are in timing and termination. Claude reaches all
three solves earliest, at mean turns 1.85, 3.62, and 6.63. Qwen uses the most turns,
averaging 13.61, reaches its first full solve latest, and reaches the
horizon without an explicit stop in 35.3\% of contexts against 0.2\% for GPT.
Qwen also has the largest zero-solve fallback count, 20 contexts compared with 5 for
GPT.

\begin{table}[!t]
\centering
\scriptsize
\setlength{\tabcolsep}{3pt}
\renewcommand{\arraystretch}{1.06}
\begin{tabular*}{\columnwidth}{@{\extracolsep{\fill}}llcccc@{}}
\toprule
Backbone & Control family & Step & Factor & Final & Mean \\
\midrule
GPT-5.6 Sol & Target coverage        & 31.9\% & 1.14$\times$ & 91.4\% & 1.884 \\
            & Serial-OAR sparing     & 33.2\% & 1.19$\times$ & 87.5\% & 0.576 \\
            & Mean-dose OAR sparing  & 32.8\% & 1.19$\times$ & 92.9\% & 1.474 \\
            & Falloff / post.\ neck  & 44.4\% & 1.25$\times$ & 89.1\% & 0.696 \\
\addlinespace[2pt]
Claude Sonnet 5 & Target coverage        & 23.8\% & 1.05$\times$ & 81.7\% & 1.840 \\
            & Serial-OAR sparing     & 20.9\% & 1.08$\times$ & 58.9\% & 1.018 \\
            & Mean-dose OAR sparing  & 32.8\% & 1.10$\times$ & 70.0\% & 1.697 \\
            & Falloff / post.\ neck  & 19.1\% & 1.07$\times$ & 29.6\% & 1.010 \\
\addlinespace[2pt]
Qwen3.6-27B & Target coverage        & 42.7\% & 1.20$\times$ & 90.0\% & 2.653 \\
            & Serial-OAR sparing     & 34.5\% & 1.21$\times$ & 74.4\% & 1.407 \\
            & Mean-dose OAR sparing  & 38.5\% & 1.24$\times$ & 80.1\% & 1.837 \\
            & Falloff / post.\ neck  & 53.6\% & 1.39$\times$ & 66.2\% & 1.434 \\
\bottomrule
\end{tabular*}
\caption{\textbf{Weight-update behavior by control family and backbone.} ``Step'' is the fraction of consecutive accepted proposals in which a control changes by more than 5\%, averaged across the family. ``Factor'' is the typical multiplicative change across consecutive accepted proposals, as in Table~\ref{tab:supp_weight_movement}. ``Final'' compares the last accepted proposal's weight vector with the all-ones initialization, and ``Mean'' is the mean final proposal weight.}
\label{tab:supp_backbone_weights}
\end{table}

The edit policies also differ. Claude makes the smallest and least persistent
changes, moving the falloff and posterior-neck controls on 19.1\% of steps and
leaving 70.4\% of those controls within 5\% of 1.0 at the end. Qwen edits most often and
most aggressively, with a 1.39$\times$ typical factor on the shaping controls
and the highest mean final weights in every family. GPT falls between the two in
step magnitude but moves every family persistently, ending more than 5\% away
from the all-ones initialization on 87.5--92.9\% of controls. These are
descriptive differences in policy, not causal explanations of the endpoint gap.
