# Supplementary material for: RadOncGym: An Agent-Based Framework for Radiotherapy Dose-Mimicking Optimization
Source: arXiv:2611.33821 source file (2026-11-25)
Supplement: Supplementary file 2 [file agent_observation.tex]

\section{Agent Observation and Public Context}
\label{supp:agent_observation}

\subsection{Public Case Description}

Every context is initialized with a public case description serialized into the
first model request, both as a flat 297-value vector and as a nested readable
JSON object. It is derived from the CT, structure masks, possible-dose mask, and
the selected model prediction, and never loads the patient reference dose. The
vector comprises the four blocks in Table~\ref{tab:supp_context_vector}.

\begin{table}[!t]
\centering
\small
\resizebox{\columnwidth}{!}{%
\begin{tabular}{@{}lcc@{}}
\toprule
\textbf{Block} & \textbf{Dim.} & \textbf{Index} \\
\midrule
Global anatomy and prediction summaries & 22  & 0--21 \\
Ten structures $\times$ 17 features     & 170 & 22--191 \\
Overlap, 7 OARs $\times$ 3 PTVs $\times$ 4 & 84 & 192--275 \\
Prediction-set identity                  & 21  & 276--296 \\
\midrule
\textbf{Total}                           & \textbf{297} & \\
\bottomrule
\end{tabular}}
\caption{\textbf{Blocks of the 297-value public context vector.} Indices are
zero-based and give the position of each block within the serialized vector.}
\label{tab:supp_context_vector}
\end{table}

The code includes the full per-index feature list.
The global block contains per-axis voxel spacing, voxel volume, possible-dose
mask voxel count and volume, eight summary statistics of the stored CT grid, and
the same eight summaries of predicted dose within the possible-dose mask.
Summary statistics are always ordered minimum, mean, maximum, p01, p05, median,
p95, and p99.

Structures appear in the order Brainstem, SpinalCord, RightParotid, LeftParotid,
Esophagus, Larynx, Mandible, PTV56, PTV63, PTV70. Each contributes a presence
flag, voxel count, volume in cm\textsuperscript{3}, a normalized centroid, three
bounding-box extents in mm, and eight predicted-dose summaries within the
structure. A missing structure is retained at fixed length with presence flag 0
and zeroed geometry and dose features.

Each OAR--PTV pair contributes intersection volume, the fraction of the OAR
overlapping the PTV, the fraction of the PTV overlapping the OAR, and their Dice
coefficient. Centroids are mean voxel coordinates divided by
$\text{grid shape}-1$ per axis; bounding boxes are inclusive voxel extents
scaled by voxel spacing; empty-region fractions and Dice values are set to 0.

\subsection{Protocol and Criterion Margins}

Every prompt lists the ten clinical criteria from the main paper.
Prescriptions of 56, 63, and 70~Gy are
implicit in the PTV names rather than given as a separate table; the prompt
states the evaluated thresholds directly. A patient-specific goal-deviation
table reports each applicable criterion's predicted value and margin,
approximating target $D_{99}$ by predicted-dose p01, serial-OAR
$D_{0.1\mathrm{cc}}$ by p99, and mean-dose criteria by the predicted mean. The
table includes only criteria whose structures are present. These percentile
substitutions are agent-facing display heuristics rather than scored quantities:
the percentile corresponding to $0.1$~cc depends on structure volume, so p99 is
not in general equal to $D_{0.1\mathrm{cc}}$. Every reported clinical-criterion
result is computed from the criterion definitions of the main paper on the
full-solve dose.

\subsection{DVH Feedback}

In the main agent conditions a DVH diagram is attached only after a successful
full solve; no image is supplied on surrogate-only turns, including every turn
before the first successful solve. The image is a PNG showing the whole-volume
predicted curves together with the optimized-plan curves, and it is updated
after each further successful solve; the candidate critic receives the same
image when reviewing a proposal. The predicted DVH is not duplicated
numerically. After a full solve, textual feedback reports exact whole-plan DVH
endpoints, per-criterion violations, plan maximum dose, homogeneity,
conformity, spill, and falloff. The fixed clinical-only condition receives no
image and no per-criterion detail.

\subsection{Structured Action Interface}

Each planner response is parsed as a structured object that is either a proposal
carrying the 12-dimensional weight vector and a binary full-solve request, or a
stop action. The weights follow the control order in
Table~\ref{tab:supp_controls} and are constrained to $[0.25,4.0]$. In the fixed
clinical-only condition, the environment enforces 13 surrogate evaluations followed
by three full solves, so the model cannot alter full-solve timing. The candidate critic does not emit replacement weights: it either accepts
the proposed action or requests one planner revision, after which the revised
structured action is executed.

\subsection{Prompt Construction, Schemas, and Retries}

The system instruction identifies the task as radiotherapy objective-weight planning; explains that weights are relative priorities rather than dose prescriptions; distinguishes approximate surrogate feedback from full-solve feedback; directs the model to preserve target coverage while considering OAR trade-offs; and requires one structured action without free-form text. The prompt instructions and JSON templates are shown in Section~\ref{supp:prompt_interface}.

The planner object contains exactly three top-level fields: \texttt{action}, \texttt{request\_full\_verifier}, and \texttt{weights}. A proposal requires all 12 named finite weights and forbids additional properties; a stop requires a false full-request bit and null weights. The environment rejects unknown controls, incomplete vectors, out-of-range values, illegal stop/full combinations, and actions exceeding the remaining budget. The candidate critic returns an accept-or-revise verdict, typed issues, revision guidance, an assessment of the proposed full request, and a confidence level.

Validation, transport-retry, and structured-output settings are given in Section~\ref{supp:prompt_overview_validation}. The traces contain no structured-output parse errors, invalid executed actions, or memory-integrity errors.

\subsection{Information Withheld from the Agent}

The patient reference dose, expert plan, DVH score, and dose score are withheld
from the agent throughout, as are the all-ones plan and its absolute objective
value. Surrogate feedback is expressed relative to that baseline, so the agent
observes differences from it without observing the baseline itself.
The all-ones plan is solved once per context, outside every method's full-solve
budget, and its result is not exposed to the language agents: it serves as the
evaluation reference and as the fallback when no full solve succeeds. The
Adaptive LogEI control is the sole condition that additionally receives the
clinical objective of that solve, which its promotion rule requires in order to
calibrate surrogate values against full-solve outcomes; this is an information
asymmetry in favor of that control relative to the agents.
