# Supplementary material for: RadOncGym: An Agent-Based Framework for Radiotherapy Dose-Mimicking Optimization
Source: arXiv:2611.33821 source file (2026-11-25)
Supplement: Supplementary file 3 [file baselines_and_controls.tex]

\section{Baseline Quality and Controller Rules}
\label{supp:baselines_controls}

\subsection{All-Ones Baseline Plan Quality by Prediction Set}

Table~\ref{tab:supp_baseline_by_set} reports the comparison referenced in the main paper, based on the plan generated with all 12 weights fixed at one. It therefore measures \emph{baseline plan quality}, which reflects both the upstream prediction and the downstream dose-mimicking solve rather than the prediction alone. Each row contains the same 60 patients under one ranked prediction set. Lower values are better, and intervals resample patients with 10,000 bootstrap replicates. Baseline plan quality is close to uniform across the ten sets: clinical-criterion violation spans 1.597--1.726~Gy with every interval overlapping. The DVH score varies more, from 4.093~Gy for set 3 to 5.244~Gy for set 7.

\begin{table*}[!t]
\centering
\footnotesize
\setlength{\tabcolsep}{3.5pt}
\begin{tabular*}{\textwidth}{@{\extracolsep{\fill}}c rr rr rr@{}}
\toprule
& \multicolumn{2}{c}{Clinical-criterion violation (Gy)}
& \multicolumn{2}{c}{DVH score (Gy)}
& \multicolumn{2}{c}{Dose score (Gy)} \\
\cmidrule(lr){2-3}\cmidrule(lr){4-5}\cmidrule(lr){6-7}
Set & Mean & 95\% CI & Mean & 95\% CI & Mean & 95\% CI \\
\midrule
1  & 1.654 & $[1.279,2.055]$ & 4.227 & $[3.827,4.658]$ & 3.332 & $[3.018,3.662]$ \\
2  & 1.667 & $[1.309,2.046]$ & 4.812 & $[4.375,5.303]$ & 3.458 & $[3.157,3.789]$ \\
3  & 1.653 & $[1.286,2.055]$ & 4.093 & $[3.652,4.563]$ & 3.270 & $[2.976,3.602]$ \\
4  & 1.661 & $[1.302,2.059]$ & 4.260 & $[3.860,4.685]$ & 3.313 & $[3.026,3.615]$ \\
5  & 1.655 & $[1.288,2.041]$ & 4.327 & $[3.832,4.839]$ & 3.328 & $[3.031,3.653]$ \\
6  & 1.667 & $[1.321,2.039]$ & 5.055 & $[4.529,5.630]$ & 3.472 & $[3.168,3.809]$ \\
7  & 1.726 & $[1.368,2.110]$ & 5.244 & $[4.728,5.804]$ & 3.561 & $[3.247,3.909]$ \\
8  & 1.601 & $[1.234,1.985]$ & 4.372 & $[3.942,4.835]$ & 3.411 & $[3.108,3.745]$ \\
9  & 1.627 & $[1.265,2.013]$ & 4.423 & $[3.954,4.911]$ & 3.427 & $[3.129,3.755]$ \\
10 & 1.597 & $[1.224,1.985]$ & 4.176 & $[3.708,4.688]$ & 3.242 & $[2.943,3.580]$ \\
\bottomrule
\end{tabular*}
\caption{\textbf{Context-matched all-ones baseline plan quality across the ten OpenKBP-Opt prediction sets.} Set identifiers follow the official rank order. The rows are repeated predictions on the same 60 anatomies and are not independent cohorts.}
\label{tab:supp_baseline_by_set}
\end{table*}

Table~\ref{tab:supp_baseline_terciles} stratifies contexts into thirds by all-ones dose score and reports the GPT gain in each third, together with the Spearman correlation between the baseline dose score and the gain. Clinical-criterion and DVH gains show no monotone trend across the thirds, whereas the dose gain is concentrated in the third with the worst baseline.

\begin{table}[!t]
\centering
\small
\setlength{\tabcolsep}{4pt}
\begin{tabular*}{\columnwidth}{@{\extracolsep{\fill}}lcccc@{}}
\toprule
Tercile & Baseline dose score & $\Delta$Clin & $\Delta$DVH & $\Delta$Dose \\
\midrule
Lowest  & 2.205 & 0.666 & 0.717 & 0.096 \\
Middle  & 3.187 & 0.566 & 0.529 & 0.083 \\
Highest & 4.752 & 0.607 & 0.550 & 0.482 \\
\midrule
Spearman $\rho$ & --- & $-0.127$ & $-0.160$ & $+0.342$ \\
\bottomrule
\end{tabular*}
\caption{\textbf{GPT-5.6 Sol gain by all-ones baseline difficulty.} Contexts are split into thirds by all-ones dose score. All entries except the Spearman $\rho$ row are in Gy. The final row is the Spearman correlation between a context's baseline dose score and its gain on that endpoint.}
\label{tab:supp_baseline_terciles}
\end{table}

\subsection{Common Action and Final-Selection Rules}

Every accepted proposal is a 12-weight vector in $[0.25,4.0]^{12}$. The environment scores every accepted vector with the surrogate verifier and sends the identical vector to Gurobi when a full solve is scheduled and budget remains. The fixed clinical-only control is the one exception: its turn 14--16 proposals are sent directly to Gurobi and are not surrogate-scored. Every accepted proposal in every other condition receives a surrogate estimate. Final selection is deterministic: among successful full solves, select the plan with the smallest mean clinical-criterion violation and break an exact tie in favor of the earlier step. Surrogate predictions cannot directly become final plans. If no full solve succeeds, reporting uses the predefined all-ones fallback. DVH and dose scores are computed only after this selection is frozen.

The full-solve budget counts requested attempts rather than successful outcomes,
identically for the agents and the non-agent methods. Every accepted
full-verifier request consumes one budget unit, including attempts that time out
or return another solver failure. A successful exact-cache replay likewise
consumes one logical unit although it performs no new physical solve, and
runtime accounting charges it the stored original solver time rather than its
replay latency. Timeouts are charged their observed elapsed solver time up to
the 1800-s limit. The precomputed all-ones reference is excluded from the method
budget and reported separately. Attempted and successful calls are tracked
separately: the three-solve GPT campaign issues 1,765 requests and records 1,732
successful solves, and the per-episode counts in
Section~\ref{supp:agent_behavior} are successes.

\subsection{Non-Agent Method Policies}

Table~\ref{tab:supp_numerical_policies} summarizes how each non-agent method proposes
candidates and what it observes in return.

\begin{table}[!t]
\centering
\scriptsize
\setlength{\tabcolsep}{2.5pt}
\begin{tabular*}{\columnwidth}{@{\extracolsep{\fill}}P{0.18\columnwidth}P{0.35\columnwidth}P{0.39\columnwidth}@{}}
\toprule
Policy & Proposal model & Observation and update \\
\midrule
Sobol & Seeded scrambled low-discrepancy sequence in bounded log-weight space, anchored at the all-ones initialization. & Outcome-independent sequence; no model update. \\
CMA-ES & \texttt{pycma} ask/tell in normalized log-weight space. & Complete weight vectors; minimizes $-\Delta J_{\mathrm{clin}}$ and updates after evaluating a population. \\
Exact-GP LogEI & All-ones-centered Sobol design, then exact Mat\'ern-5/2 ARD GP with LogEI. & Patient-local weight/scalar pairs; maximizes log expected improvement in $\Delta J_{\mathrm{clin}}$. \\
SAAS-BO & Sobol initialization, then fully Bayesian sparse-axis GP with qLogEI. & Weight/scalar pairs; maximizes $\Delta J_{\mathrm{clin}}$ by NUTS inference and Monte Carlo acquisition. \\
\bottomrule
\end{tabular*}
\caption{\textbf{Non-agent proposal policies.} The numerical optimizers are not directly provided CT features, structure summaries, criterion-level feedback, or DVH diagrams; the shared surrogate verifier that scores their proposals does consume anatomical and predicted-dose features.}
\label{tab:supp_numerical_policies}
\end{table}

In the standard three-solve comparison, all four methods use the 16-turn protocol reported in the main paper: 13 surrogate-screening turns followed by three terminal full solves of the best distinct unverified candidates. A full-solve outcome may enter an optimizer's state on the turn it is returned, but it cannot change which candidate is promoted afterwards. The three terminal candidates are fixed by surrogate rank at the end of screening, and each of turns 14--16 promotes the next-best remaining candidate in that order, so an earlier full-solve result never changes which candidate is promoted later. Interleaving full-solve outcomes into subsequent proposals requires the explicit fidelity-selection controller of the Adaptive LogEI control. The fixed clinical-only GPT control uses the same schedule and scalar clinical feedback, while retaining the named 12-control descriptions and iterative language policy. Surrogate-evaluation counts are therefore matched alongside horizons: every method in this comparison receives 13 surrogate evaluations and three full-solve attempts per context. That control proposes a complete weight vector on all 16 turns, but its turn 14--16 proposals are solved directly rather than surrogate-scored. One difference remains, and it favors the control. At each full-solve turn it generates a new candidate conditioned on the full-solve outcomes observed so far, whereas the non-agent methods promote candidates fixed by surrogate rank at the end of screening. The fixed clinical-only control therefore retains adaptive use of full-solve feedback that the non-agent methods do not have, while matching them on horizon, surrogate-evaluation count, solve budget, and scalar feedback. Extended Exact-GP LogEI uses 61 surrogate turns followed by three full-solve attempts, for 64 turns total.

In the 16-solve condition the schedule contains no surrogate-screening turns: each of the 16 turns is full-solved. Every turn therefore returns the full-solve $\Delta J_{\mathrm{clin}}$, no surrogate score enters these methods' updates, and the condition is a single-fidelity optimization over 16 evaluations rather than a screen-then-verify schedule.

At both solve budgets, each non-agent optimizer exposes a single scalar channel and receives one value per turn: the surrogate-verifier prediction of $\Delta J_{\mathrm{clin}}$ on a surrogate turn and the full-solve $\Delta J_{\mathrm{clin}}$ on a full-solve turn. Both are improvements over the context-matched all-ones plan in the reported convention of Section~\ref{supp:reproducibility}, so the scalar channel has a single orientation throughout and higher is always better. It receives no per-criterion, DVH, or dose information at either fidelity. CMA-ES updates its population statistics, Exact-GP LogEI and SAAS-BO condition their surrogate models, and Sobol advances its sequence, each using whichever scalar the turn returned. The optimizers differ only in the sign they require internally: the LogEI and qLogEI acquisitions of Exact-GP LogEI and SAAS-BO maximize and therefore consume $\Delta J_{\mathrm{clin}}$ directly; CMA-ES minimizes by construction and is passed $-\Delta J_{\mathrm{clin}}$; and Sobol consumes no outcome at all. No other transformation is applied at either budget. Consistent with Section~\ref{supp:reproducibility}, none of the four models the two sources as distinct fidelities and none selects fidelity online; the schedule fixes which fidelity a turn uses. The 16-solve rows of the main comparison table use the optimizer configurations of Table~\ref{tab:supp_optimizer_settings}, unchanged from the three-solve rows.

\paragraph{Adaptive LogEI.}
This control uses a 16-turn horizon and at most three full solves; promoting a candidate to a full solve does not consume an additional turn. It first reads the full solve of the all-ones anchor, which is precomputed once per context and excluded from every method's budget, so all three of its own full solves remain available. For later candidates it estimates the mean observed discrepancy between full and surrogate clinical objectives and forms
\begin{equation}
\Delta\widehat{J}_{\mathrm{full}}(w)=\Delta J_{\mathrm{sur}}(w)+
\operatorname{mean}_{v\in\mathcal{V}}
\left[\Delta J_{\mathrm{full}}(v)-\Delta J_{\mathrm{sur}}(v)\right],
\end{equation}
where $\mathcal{V}$ is the set of successfully verified candidates. It promotes the unverified candidate with the largest calibrated value when that value improves on the best observed full-solve value. When the remaining turn count equals the remaining full budget, it promotes the best eligible unverified candidates to avoid leaving legal calls unused. Thus Adaptive LogEI can incorporate each successful Gurobi outcome before later proposals, while retaining a scalar observation and deterministic fidelity-selection rule.

\paragraph{Upper-budget reference.}
The 16-full-solve condition holds the 16-turn agent architecture fixed while allowing every proposed candidate to receive a Gurobi solve. It estimates performance headroom when the full-solve bottleneck is relaxed; it is not part of the matched three-solve comparison.
