# Supplementary material for: RadOncGym: An Agent-Based Framework for Radiotherapy Dose-Mimicking Optimization
Source: arXiv:2611.33821 source file (2026-11-25)
Supplement: Supplementary file 4 [file clinical_safety.tex]

\section{Clinical-Criterion Satisfaction and Violation Details}
\label{supp:clinical_safety}

Individual-criterion satisfaction pools all applicable criterion decisions, whereas strict all-criteria feasibility requires every applicable clinical criterion for a plan to be satisfied within a $10^{-9}$ Gy numerical tolerance. Strict feasibility here means simultaneous satisfaction of the benchmark clinical criteria; it does not refer to feasibility of the inner linear program, in which these criteria are not constraints (Section~\ref{supp:planning_formulation}).
Structures absent for a patient are excluded from both pass and failure denominators.
For the per-criterion summaries below, each entry is \emph{violation rate / median positive violation / 95th-percentile positive violation}; the latter two quantities are in Gy and are shown with em dashes when no positive violations exist.
The intervals in Table~\ref{tab:supp_safety_summary}(b) are marginal patient-clustered intervals for each method separately; Section~\ref{supp:uncertainty} reports paired comparisons for the three improvement endpoints; no paired interval is computed for strict feasibility.

Table~\ref{tab:supp_safety_criterion_main} compares the principal methods criterion by criterion, and Table~\ref{tab:supp_safety_gpt} gives the same breakdown for the nine GPT-5.6 Sol memory--role configurations.
Across all nine configurations, brainstem, spinal cord, mandible, and esophagus are satisfied in every context in which the structure is present, and the target criteria differ little, so the configurations separate almost entirely on parotid and larynx violation rates. The evaluator planner has the highest violation rate on both parotids under all three memory mechanisms, which is the same ordering as the paired intervals in Section~\ref{supp:uncertainty}. The gain is concentrated in the organs at risk: target-coverage violation
rates rise slightly for GPT-5.6 Sol, from 48.3\% to 50.2\% on PTV70 and from
10.3\% to 11.3\% on PTV63, even though the PTV70 weight is raised in most
contexts.

\begin{table*}[!tbp]
\centering
\small
\textbf{(a) Aggregate criterion satisfaction}\par\smallskip
\setlength{\tabcolsep}{5pt}
\begin{tabular*}{\textwidth}{@{\extracolsep{\fill}}lrrrr@{}}
\toprule
Plan & Satisfied criteria & Satisfaction & Fully feasible plans & Strict feasibility \\
\midrule
Expert reference & 370/502 & 73.7\% & 9/60 & 15.0\% \\
All ones & 3912/5020 & 77.9\% & 78/600 & 13.0\% \\
GPT-5.6 Sol & 4117/5020 & 82.0\% & 123/600 & 20.5\% \\
\bottomrule
\end{tabular*}

\medskip
\textbf{(b) Selected-plan largest remaining violations}\par\smallskip
\setlength{\tabcolsep}{4pt}
\begin{tabular*}{\textwidth}{@{\extracolsep{\fill}}lrrrrr@{}}
\toprule
Method & Strict feasibility & Patient-clustered 95\% CI & Mean & Median & P95 \\
\midrule
All ones & 13.0\% & $[6.3,20.5]$ & 10.01 & 8.37 & 27.77 \\
Sobol-3 & 14.3\% & $[7.3,22.0]$ & 9.58 & 7.24 & 27.77 \\
CMA-ES-3 & 14.7\% & $[7.8,22.3]$ & 9.63 & 7.32 & 27.58 \\
Exact-GP-3 & 13.7\% & $[7.0,21.0]$ & 9.14 & 7.23 & 25.53 \\
SAAS-BO-3 & 16.2\% & $[8.8,24.2]$ & 8.83 & 6.95 & 26.05 \\
Adaptive LogEI & 17.5\% & $[9.7,25.8]$ & 8.32 & 5.57 & 25.43 \\
GPT & 20.5\% & $[12.3,29.5]$ & 6.65 & 3.68 & 24.63 \\
Claude & 18.7\% & $[10.7,27.5]$ & 7.22 & 4.41 & 24.68 \\
Qwen & 18.5\% & $[10.5,27.5]$ & 7.79 & 5.12 & 25.02 \\
\bottomrule
\end{tabular*}
\caption{\textbf{Aggregate constraint-satisfaction results.} The largest-remaining-violation statistics in (b) are in Gy. The expert reference contains one plan per patient; repeating it across ten prediction contexts leaves its percentages unchanged. The SAAS-BO-3 row uses 590 audited selections and 10 predefined all-ones fallbacks.}
\label{tab:supp_safety_summary}
\end{table*}

\begin{table*}[!tbp]
\centering
\scriptsize
\setlength{\tabcolsep}{3pt}
\renewcommand{\arraystretch}{1.04}
\textbf{(a) Violation rate (\%) / median positive violation (Gy)}\par\smallskip
\begin{tabular*}{\textwidth}{@{\extracolsep{\fill}}lccccccccc@{}}
\toprule
Criterion & All ones & Sobol-3 & CMA-ES-3 & Exact-GP-3 & SAAS-BO-3 & Adaptive & GPT & Claude & Qwen \\
\midrule
Brainstem & 0.0 / \textemdash{} & 0.0 / \textemdash{} & 0.0 / \textemdash{} & 0.0 / \textemdash{} & 0.0 / \textemdash{} & 0.0 / \textemdash{} & 0.0 / \textemdash{} & 0.0 / \textemdash{} & 0.0 / \textemdash{} \\
Spinal cord & 0.2 / 0.23 & 0.2 / 0.23 & 0.2 / 0.23 & 0.2 / 0.21 & 0.4 / 0.45 & 1.1 / 0.78 & 0.0 / \textemdash{} & 0.0 / \textemdash{} & 0.0 / \textemdash{} \\
Mandible & 0.0 / \textemdash{} & 0.0 / \textemdash{} & 0.0 / \textemdash{} & 0.0 / \textemdash{} & 0.0 / \textemdash{} & 0.0 / \textemdash{} & 0.0 / \textemdash{} & 0.0 / \textemdash{} & 0.0 / \textemdash{} \\
Right parotid & 54.2 / 7.45 & 53.6 / 7.40 & 47.1 / 6.85 & 53.1 / 7.18 & 47.3 / 6.89 & 39.3 / 5.98 & 34.6 / 4.37 & 41.7 / 4.46 & 41.5 / 5.66 \\
Left parotid & 55.8 / 9.03 & 52.0 / 7.99 & 58.5 / 8.68 & 49.8 / 7.51 & 51.4 / 7.83 & 50.3 / 7.15 & 41.7 / 5.17 & 45.3 / 5.80 & 45.4 / 6.95 \\
Esophagus & 0.0 / \textemdash{} & 0.0 / \textemdash{} & 0.0 / \textemdash{} & 0.0 / \textemdash{} & 0.0 / \textemdash{} & 0.4 / 0.22 & 0.0 / \textemdash{} & 0.0 / \textemdash{} & 0.0 / \textemdash{} \\
Larynx & 28.7 / 9.08 & 27.5 / 8.60 & 32.2 / 8.60 & 30.9 / 9.69 & 25.0 / 9.51 & 26.6 / 10.02 & 21.6 / 8.45 & 24.1 / 8.23 & 23.8 / 8.53 \\
PTV56 & 2.3 / 0.52 & 2.3 / 0.40 & 2.2 / 0.53 & 2.2 / 0.42 & 3.0 / 0.40 & 2.8 / 0.41 & 2.5 / 0.40 & 2.7 / 0.49 & 2.7 / 0.53 \\
PTV63 & 10.3 / 1.12 & 9.8 / 1.06 & 9.7 / 1.43 & 10.0 / 1.00 & 10.3 / 1.38 & 10.7 / 1.35 & 11.3 / 1.03 & 10.8 / 1.33 & 9.8 / 1.59 \\
PTV70 & 48.3 / 2.42 & 47.7 / 2.44 & 48.2 / 2.39 & 48.2 / 2.35 & 49.7 / 2.31 & 49.8 / 2.45 & 50.2 / 2.62 & 51.0 / 2.43 & 50.0 / 2.42 \\
\bottomrule
\end{tabular*}

\medskip
\textbf{(b) P95 positive violation (Gy)}\par\smallskip
\begin{tabular*}{\textwidth}{@{\extracolsep{\fill}}lccccccccc@{}}
\toprule
Criterion & All ones & Sobol-3 & CMA-ES-3 & Exact-GP-3 & SAAS-BO-3 & Adaptive & GPT & Claude & Qwen \\
\midrule
Brainstem & \textemdash{} & \textemdash{} & \textemdash{} & \textemdash{} & \textemdash{} & \textemdash{} & \textemdash{} & \textemdash{} & \textemdash{} \\
Spinal cord & 0.23 & 0.23 & 0.23 & 0.21 & 0.71 & 1.33 & \textemdash{} & \textemdash{} & \textemdash{} \\
Mandible & \textemdash{} & \textemdash{} & \textemdash{} & \textemdash{} & \textemdash{} & \textemdash{} & \textemdash{} & \textemdash{} & \textemdash{} \\
Right parotid & 27.94 & 27.96 & 27.61 & 27.51 & 26.27 & 25.43 & 25.11 & 25.11 & 25.80 \\
Left parotid & 28.15 & 28.11 & 28.24 & 26.00 & 26.66 & 28.22 & 25.03 & 25.34 & 25.69 \\
Esophagus & \textemdash{} & \textemdash{} & \textemdash{} & \textemdash{} & \textemdash{} & 0.22 & \textemdash{} & \textemdash{} & \textemdash{} \\
Larynx & 25.09 & 25.10 & 25.06 & 25.26 & 25.11 & 25.09 & 24.74 & 24.96 & 24.92 \\
PTV56 & 1.96 & 1.62 & 1.46 & 1.52 & 1.27 & 1.87 & 1.69 & 1.79 & 1.59 \\
PTV63 & 4.73 & 4.84 & 4.96 & 4.56 & 5.08 & 5.12 & 5.16 & 4.89 & 5.21 \\
PTV70 & 9.00 & 7.54 & 8.69 & 8.68 & 8.23 & 8.55 & 8.30 & 8.87 & 8.20 \\
\bottomrule
\end{tabular*}
\caption{\textbf{Per-criterion comparison across principal methods.} Em dashes indicate that no positive violation occurred. Adaptive, GPT, Claude, and Qwen abbreviate Adaptive LogEI, GPT-5.6 Sol, Claude Sonnet 5, and Qwen3.6-27B; the $-3$ suffix marks the three-solve condition.}
\label{tab:supp_safety_criterion_main}
\end{table*}

\begin{table*}[!tbp]
\centering
\footnotesize
\setlength{\tabcolsep}{6pt}
\renewcommand{\arraystretch}{1.10}
\begin{tabular*}{\textwidth}{@{\extracolsep{\fill}}lccc@{}}
\toprule
Criterion & Direct planner & Evaluator planner & Candidate critic \\
\midrule
\multicolumn{4}{@{}l}{\bfseries Lossless full-history memory} \\
Brainstem & 0.0/\textemdash{} / \textemdash{} & 0.0/\textemdash{} / \textemdash{} & 0.0/\textemdash{} / \textemdash{} \\
Spinal cord & 0.0/\textemdash{} / \textemdash{} & 0.0/\textemdash{} / \textemdash{} & 0.0/\textemdash{} / \textemdash{} \\
Mandible & 0.0/\textemdash{} / \textemdash{} & 0.0/\textemdash{} / \textemdash{} & 0.0/\textemdash{} / \textemdash{} \\
Right parotid & 33.6/4.37 / 24.83 & 37.3/4.73 / 24.96 & 34.7/4.27 / 24.75 \\
Left parotid & 40.5/5.07 / 25.13 & 42.7/5.79 / 25.71 & 41.2/5.54 / 25.25 \\
Esophagus & 0.0/\textemdash{} / \textemdash{} & 0.0/\textemdash{} / \textemdash{} & 0.0/\textemdash{} / \textemdash{} \\
Larynx & 22.2/7.95 / 24.73 & 22.2/8.96 / 24.82 & 22.8/7.88 / 24.65 \\
PTV56 & 2.8/0.36 / 1.82 & 2.7/0.30 / 1.75 & 2.8/0.44 / 1.48 \\
PTV63 & 11.0/1.26 / 5.84 & 11.0/1.16 / 4.62 & 10.8/1.15 / 5.67 \\
PTV70 & 51.3/2.50 / 8.45 & 50.7/2.33 / 8.49 & 50.8/2.52 / 8.03 \\
\addlinespace[2pt]
\multicolumn{4}{@{}l}{\bfseries Criterion-response contrast memory} \\
Brainstem & 0.0/\textemdash{} / \textemdash{} & 0.0/\textemdash{} / \textemdash{} & 0.0/\textemdash{} / \textemdash{} \\
Spinal cord & 0.0/\textemdash{} / \textemdash{} & 0.0/\textemdash{} / \textemdash{} & 0.0/\textemdash{} / \textemdash{} \\
Mandible & 0.0/\textemdash{} / \textemdash{} & 0.0/\textemdash{} / \textemdash{} & 0.0/\textemdash{} / \textemdash{} \\
Right parotid & 33.9/4.27 / 24.92 & 37.5/4.76 / 25.01 & 34.6/4.37 / 25.11 \\
Left parotid & 40.2/5.06 / 25.14 & 43.2/5.72 / 25.62 & 41.7/5.17 / 25.03 \\
Esophagus & 0.0/\textemdash{} / \textemdash{} & 0.0/\textemdash{} / \textemdash{} & 0.0/\textemdash{} / \textemdash{} \\
Larynx & 23.1/7.67 / 24.74 & 23.8/8.23 / 24.89 & 21.6/8.45 / 24.74 \\
PTV56 & 2.3/0.63 / 1.76 & 2.5/0.48 / 1.69 & 2.5/0.40 / 1.69 \\
PTV63 & 11.0/1.04 / 5.48 & 11.0/1.11 / 5.05 & 11.3/1.03 / 5.16 \\
PTV70 & 49.8/2.49 / 8.43 & 50.7/2.37 / 8.62 & 50.2/2.62 / 8.30 \\
\addlinespace[2pt]
\multicolumn{4}{@{}l}{\bfseries Pareto-tradeoff memory} \\
Brainstem & 0.0/\textemdash{} / \textemdash{} & 0.0/\textemdash{} / \textemdash{} & 0.0/\textemdash{} / \textemdash{} \\
Spinal cord & 0.0/\textemdash{} / \textemdash{} & 0.0/\textemdash{} / \textemdash{} & 0.0/\textemdash{} / \textemdash{} \\
Mandible & 0.0/\textemdash{} / \textemdash{} & 0.0/\textemdash{} / \textemdash{} & 0.0/\textemdash{} / \textemdash{} \\
Right parotid & 34.4/4.56 / 24.72 & 36.6/4.86 / 25.12 & 35.4/4.27 / 24.25 \\
Left parotid & 41.4/5.16 / 25.12 & 43.9/5.93 / 25.64 & 40.7/5.47 / 25.35 \\
Esophagus & 0.0/\textemdash{} / \textemdash{} & 0.0/\textemdash{} / \textemdash{} & 0.0/\textemdash{} / \textemdash{} \\
Larynx & 23.4/7.31 / 24.65 & 22.5/8.41 / 24.96 & 23.8/7.57 / 24.76 \\
PTV56 & 2.7/0.35 / 2.24 & 2.7/0.39 / 1.49 & 2.7/0.45 / 1.86 \\
PTV63 & 11.0/1.36 / 4.72 & 10.7/1.14 / 4.70 & 11.2/1.31 / 5.18 \\
PTV70 & 51.0/2.50 / 8.88 & 50.0/2.51 / 8.74 & 50.7/2.51 / 8.64 \\
\bottomrule
\end{tabular*}
\caption{\textbf{Per-criterion results for the nine GPT-5.6 Sol memory-role configurations.} Cells report violation rate (\%) / median positive violation (Gy) / P95 positive violation (Gy).}
\label{tab:supp_safety_gpt}
\end{table*}
