# Supplementary material for: RadOncGym: An Agent-Based Framework for Radiotherapy Dose-Mimicking Optimization
Source: arXiv:2611.33821 source file (2026-11-25)
Supplement: Supplementary file 5 [file planning_formulation.tex]

\section{Planning Formulation and Objective Weights}
\label{supp:planning_formulation}

This section gives the dose-mimicking linear program summarized in the main
paper, the objective families controlled by each of the 12 weights, and the relation
between the inner planning objective and the benchmark clinical-criterion score.

\subsection{Reference Objectives from the Predicted Dose}

The planning pipeline loads the AI-predicted three-dimensional dose
map and reduces it to structure-level reference values within each anatomical
mask. Gurobi does not receive the predicted dose map itself; it receives a
linear program whose constants are these summaries. For a structure $S$ with
predicted dose $d^{\mathrm{AI}}$, the reference objectives comprise the mean
dose, the maximum dose, upper-tail dose terms for organs at risk, overdose and
underdose terms for planning target volumes, and analogous terms for target
rings and the posterior neck. We write $r_j$ for the reference value of
objective $j$.

Two families of reference structures are derived rather than supplied. For
every present PTV, 3-mm and 6-mm Euclidean expansions are formed within the
external patient contour, the PTV voxels are removed, and overlaps between
derived regions are pruned by the fixed priority rule of OpenKBP-Opt; all
objective rows belonging to these rings share the \texttt{ring\_falloff}
multiplier. The posterior-neck region is a 5-mm ring around the spinal cord, or
around the brainstem when the cord is absent. On each axial slice it retains
external-contour voxels whose lateral coordinate lies between the extrema of
that ring and whose remaining in-plane coordinate lies beyond the ring's mean
coordinate, after which all target voxels are removed. Every such objective row
maps to \texttt{posterior\_neck\_sparing}.

The formulation is therefore not a voxelwise matching loss: it does not
minimize $\sum_v |d_v - d^{\mathrm{AI}}_v|$. The predicted dose influences the
plan through its structure-level summaries.

\subsection{Absolute-Mean Dose-Mimicking Objective}

Let $x$ be the beamlet-intensity vector and $A$ the dose-influence matrix, so
that the optimized voxel dose is $d = Ax$. Each objective value $\phi_j(d)$ is
computed from these optimized voxel doses. Under the \emph{absolute-mean}
formulation used in all reported experiments, the model introduces nonnegative
deviation variables $\sigma_j$ and $\psi_j$ satisfying
%
\begin{equation}
r_j + \sigma_j - \psi_j = \phi_j(d),
\label{eq:supp_deviation}
\end{equation}
%
where $\sigma_j$ is an increase and $\psi_j$ a reduction relative to the
reference. Gurobi minimizes
%
\begin{equation}
\sum_j w_{c(j)}\left(\sigma_j - 10^{-5}\psi_j\right),
\label{eq:supp_lp_objective}
\end{equation}
%
with $w_{c(j)}$ the agent-selected weight for the control governing objective
$j$. At the optimum this is equivalent to
%
\begin{equation}
\sum_j w_{c(j)}
\left[
\max\!\left(\phi_j(d)-r_j,\,0\right)
-10^{-5}\max\!\left(r_j-\phi_j(d),\,0\right)
\right].
\label{eq:supp_equivalent}
\end{equation}
%
The formulation penalizes objectives that worsen relative to the predicted dose
and gives a small preference to those that improve. \emph{Absolute} indicates
that deviations are expressed in Gy rather than normalized by the reference
value; \emph{mean} indicates aggregation across objective components rather
than minimization of the single worst component.

\subsection{Voxel-Derived Objective Families}

For a structure $S$, the mean-dose component is
%
\begin{equation}
\mu_S(d) = \frac{1}{|S|}\sum_{v\in S} d_v,
\end{equation}
%
and the maximum-dose component is represented by an auxiliary variable
satisfying $m_S(d) \geq d_v$ for all $v \in S$. Hinge components are taken at a
fractional threshold $\tau$ of a structure-level scale $M_S$ and a sign
$s\in\{+1,-1\}$,
%
\begin{equation}
q_{S,\tau,s}(d) = \frac{1}{|S|}\sum_{v\in S}
\max\!\left(0,\,s\left(d_v-\tau M_S\right)\right),
\label{eq:supp_hinge}
\end{equation}
%
where $M_S$ is the maximum predicted dose within $S$ for an organ at risk and
the prescription $p_S\in\{56,63,70\}$~Gy for a target. Organs at risk carry
upper-tail terms, $s=+1$, at
%
\begin{equation}
\tau\in\{0.975,\,0.90,\,0.75,\,0.50,\,0.25\}.
\end{equation}
%
Targets carry two terms: overdose at $(\tau,s)=(1.05,+1)$ and underdose at
$(\tau,s)=(1.00,-1)$. These expressions are linearized with auxiliary variables, so the planning
problem remains a linear program.

\subsection{Objective-Weight Controls}

The agent supplies one multiplier per control, listed in
Table~\ref{tab:supp_controls}. Each multiplier scales every objective component
associated with that control rather than an individual dose term. For example,
\texttt{LeftParotid\_sparing} scales the left-parotid mean-, maximum-, and
tail-dose contributions together, and \texttt{PTV70\_coverage} scales the PTV70
maximum-dose, overdose, and underdose components. Weights are bounded to
$0.25 \leq w_c \leq 4.0$. Increasing a weight gives the corresponding
objectives greater influence over the optimized beamlet intensities; decreasing
it permits more trade-off against competing structures and targets.

\begin{table}[H]
    \centering
    \small
    \setlength{\tabcolsep}{4pt}
    \renewcommand{\arraystretch}{1.08}
    \begin{tabular*}{\columnwidth}{@{\extracolsep{\fill}}>{\raggedright\arraybackslash}p{0.56\columnwidth}>{\raggedright\arraybackslash}p{0.34\columnwidth}@{}}
        \toprule
        \textbf{Control family and controls} & \textbf{Scaled terms} \\
        \midrule
        \textbf{Target coverage:} PTV56, PTV63, PTV70
        & maximum; overdose; underdose \\
        \textbf{Organ sparing:} Brainstem, spinal cord, right parotid,
        left parotid, esophagus, larynx, mandible
        & mean; maximum; upper-tail \\
        \textbf{Auxiliary regions:} ring falloff, posterior neck
        & mean; maximum; upper-tail \\
        \bottomrule
    \end{tabular*}
    \caption{\textbf{Objective-weight controls and the components each
    multiplier scales.} The action keys append
    \texttt{\_coverage} to target names and \texttt{\_sparing} to organ names;
    the two auxiliary keys are \texttt{ring\_falloff} and
    \texttt{posterior\_neck\_sparing}. All weights are bounded to
    $[0.25,4.0]$.}
    \label{tab:supp_controls}
\end{table}

\subsection{Additional Planning Constraints}

The linear program also enforces the physical fluence-to-dose relationship and
machine-related restrictions. Beamlet intensities are bounded by
$0 \leq x_j \leq 15$ and the optimization voxel doses by
$0 \leq d_i \leq 82$~Gy, subject to dose-influence consistency $d = Ax$. The
optimization voxel set is the complete set of voxels belonging to the clinical
and derived optimization structures, taken without downsampling; it is a subset
of the possible-dose grid rather than a sample drawn from it. \emph{Full
resolution} in Section~\ref{supp:reproducibility} refers to this absence of
downsampling, not to optimization over every possible-dose voxel.

Fluence complexity is limited by a sum of positive gradients. For each beamlet
$j$ an auxiliary variable satisfies
%
\begin{equation}
g_j \geq \max\!\left(0,\,x_j - x_{j+1}\right),
\end{equation}
%
taking $x_{j+1}=0$ where the right neighbor is missing. For every row $r$ of the
fluence grid at beam angle $a$, an auxiliary variable satisfies
$u_a \geq \sum_{j\in r} g_j$, and the imposed limit is $\sum_a u_a \leq 65$.
This is equivalent to
%
\begin{equation}
\sum_a \max_r \sum_{j\in r}\max\!\left(0,\,x_j - x_{j+1}\right) \leq 65.
\end{equation}
%
After optimization the fluence vector is applied to the full-resolution
dose-influence matrix, $d_{\mathrm{full}} = A_{\mathrm{full}}x$, to generate the
final dose distribution.

All remaining linear-program construction details follow OpenKBP-Opt commit
\texttt{16fbe0dbc64c94ed4b7e}\allowbreak\texttt{8378a090b47c6596bbd7}.
RadOncGym changes only the twelve groups of objective coefficients and the
solver configuration of Section~\ref{supp:reproducibility}.

\subsection{Inner and Outer Objectives}

The planning objective in Eq.~\eqref{eq:supp_equivalent} and the benchmark
objective are distinct. The criteria listed in the clinical-criteria table of
the main paper are evaluated on the generated dose after the solve and are not
imposed as hard constraints in the linear program. The objective weights
influence these criteria only indirectly through the generated dose. Thus, the
inner optimization matches predicted-dose-derived reference objectives, while
the outer benchmark evaluates clinical-criterion violations after the solve.
