# Supplementary material for: RadOncGym: An Agent-Based Framework for Radiotherapy Dose-Mimicking Optimization
Source: arXiv:2611.33821 source file (2026-11-25)
Supplement: Supplementary file 6 [file prompts.tex]

\section{Agent Prompts and Structured Interfaces}
\label{supp:prompt_interface}

The language-model interface is defined by three components: a common planner
system instruction, a turn-specific public observation, and a strict structured
output format. The observation grows as public surrogate and full-solve
results become available, but the instruction and field meanings remain fixed.
The boxes below give the prompt specification and the JSON structures
used by the planner, evaluator, and candidate critic. Angle-bracketed entries
denote turn-specific data or, when the content is itself structured, an
abbreviated sub-object. They do not indicate omitted fields.

The instruction and observation template contain conditional clauses for two
facilities that no reported experiment enabled: retrieval of training-split
examples and the memory-management budget. Neither was ever activated, and the
corresponding observation fields are absent throughout.

\subsection{Common Planner System Instruction}
\label{supp:prompt_overview_common}

The boxes below give the full common planner instruction, reformatted for
a two-column page.

\begin{promptbox}{Planner instruction: role and response format}
You are a radiotherapy objective-weight planning agent in RadOncGym. Choose
exactly one next action from the supplied JSON observation. Return one JSON
object only: no Markdown, prose outside JSON, assistant tags, copied
observation text, or hidden reasoning blocks.
\end{promptbox}

\begin{promptbox}{Planner instruction: action rules}
Obey the supplied task and action rules. For an agent-choice task, propose
one complete objective-weight vector and decide whether that identical
candidate should also receive a budgeted full physics-verifier call. For a
full-only task, every proposed candidate must request full verification. There
is no external router, and the environment does not force or rewrite an action.

\end{promptbox}

\begin{promptbox}{Planner instruction: evidence and priorities}
\textbf{Evidence and planning priorities.}
Cheap feedback is an approximate learned estimate. Full feedback comes from a
physics optimization and contains generated-plan protocol metrics, but never
hidden expert-reference errors. Lower reported objective and constraint violations are better. Preserve target coverage before pursuing discretionary
OAR gains. Use the explicitly identified memory view to avoid unproductive
duplicates. Any retrieved example comes only from public training-split
trajectories and includes its source and retrieval score.

\smallskip
\end{promptbox}

\begin{promptbox}{Planner instruction: meaning of the controls}
\textbf{Meaning of the controls.}
Interpret weights as relative priorities inside the inverse-planning objective,
not as direct dose prescriptions. Increasing a target-coverage weight raises
the relative penalty for missing that target objective. Increasing an
OAR-sparing weight raises the relative penalty attached to that OAR objective.
The ring and posterior-neck controls emphasize dose falloff and avoidance in
their derived structures. Because all effects interact through patient
geometry, infer direction from the observed weight--response history rather
than assuming independent or monotonic improvement in every metric.

\smallskip
\end{promptbox}

\begin{promptbox}{Planner instruction: use of the expensive verifier}
\textbf{Use of the expensive verifier.}
Use cheap evaluations to explore and compare candidates. A full request is
scarce and should be attached to the exact candidate whose generated-plan DVH
and protocol response would materially inform a later decision or final choice.
To escalate a previously cheap-evaluated candidate, resubmit its exact weights
with \texttt{request\_full\_verifier=true}; this deliberate duplicate is
accepted and returns cheap and full feedback for identical weights.

\smallskip
Do not request a full evaluation merely because budget remains, and do not
avoid one when cheap and observed physics evidence disagree or an important
trade-off requires confirmation. A full call on the last turn cannot guide a
revision. When several full calls are available, distribute their information
value across the remaining horizon so that at least an earlier call can inform
later proposals. The planner owns this decision.
\end{promptbox}

\begin{promptbox}{Planner instruction: memory-management rules}
If memory-management rules are present, memory operations are advisory,
evidence-checked requests with a separate budget. They become visible only on
a later turn, never replace the required planning action, and never alter the
environment's immutable public history.
\end{promptbox}

\subsection{Planner Input Object}

Each user message contains one serialized object with the following top-level
structure. Optional advisory blocks appear only in the corresponding
role or memory condition.

\begin{promptbox}{Planner input: top-level template}
\begin{promptjson}
{
  "schema_version": "<interface version>",
  "task": {
    "task_id": "<id>", "kind": "<task kind>",
    "fidelity_control": "<agent choice or full only>",
    "full_incumbent_rule": "<rule>",
    "stop_requires_evaluated_candidate": <bool>,
    "minimum_evaluated_candidates_before_stop": <int>,
    "remaining_evaluated_candidates_before_stop": <int>
  },
  "information_policy": {
    "history": "<registered memory view>",
    "hidden_reference_feedback_available": false,
    "external_router": false,
    "automatic_full_call_forcing": false,
    "feedback_sources": {<cheap, full, audit meanings>},
    "cheap_full_semantics": {<targets and alignment>}
  },
  "action_contract": {
    "objective_names_in_order": [<12 names>],
    "weight_minimum": 0.25, "weight_maximum": 4.0,
    "complete_weight_vector_required": true,
    "agent_controls_full_request": <bool>,
    "candidate_must_request_full": <bool>,
    "allowed_actions": ["propose_weights"<, "stop">]
  }
}
\end{promptjson}
\end{promptbox}

\begin{promptbox}{Planner input: public observation fields}
\begin{promptjson}
{
  "clinical_preference": {<criterion priorities>},
  "objective_semantics": {<meaning of each control>},
  "verifier_strategy": {<cheap/full roles and budget guidance>},
  "clinical_protocol": [
    {"metric": <name>, "roi": <name>,
     "relation": <upper/lower>, "threshold_gy": <value>}, ...],
  "public_case": {<case IDs, anatomy, prediction, 297 features>},
  "public_dvh": <generated-plan DVH descriptor or null>,
  "memory_view": {<selected public steps and outcomes>},
  "performance_support": {<enabled public support modules>},
  "episode_observation": {
    "context": {<public identifiers>},
    "budgets": {<steps, cheap calls, full calls remaining>},
    "incumbents": {<best cheap step, best full step>},
    "history": [<accepted/rejected actions and public outcomes>]
  },
  "planner_critique": <evaluator JSON, when enabled>,
  "planner_critique_contract": <advisory-only rules>,
  "memory_management_contract": <optional rules>
}
\end{promptjson}
\end{promptbox}

The public case contains leak-safe CT, anatomy, overlap, and predicted-dose
summaries. The history contains previous weight vectors, acceptance
status, surrogate predictions and uncertainty, successful full-solve status and
cost, optimized-plan endpoints, criterion violations, and public incumbent
pointers as applicable. In image-enabled conditions, the current optimized-plan
DVH diagram is supplied as an image alongside this object once a full solve has
succeeded. The expert
reference dose, DVH score, dose score, oracle ranks, and any
reference-derived routing signal are absent.

The task fields above take fixed values within each reported condition, though some differ across conditions. All dynamic
language-agent conditions use \texttt{full\_incumbent\_rule} =
\texttt{quality\_only}, under which the successful full-solved candidate with the
lowest mean clinical-criterion violation is selected and an exact tie is broken
in favor of the earlier step. Stopping requires at least one accepted, evaluated
candidate: \texttt{stop\_requires\_evaluated\_candidate} = \texttt{true} and
\texttt{minimum\_evaluated\_candidates\_before\_stop} = 1. Accordingly,
\texttt{remaining\_evaluated\_candidates\_before\_stop} is one at reset and zero
after the first accepted candidate evaluation, so the earliest legal stop is
turn 2; the earliest observed stop, on turn 6, reflects model behavior rather
than an environment restriction. The fixed clinical-only and 16-full-solve
conditions disable stopping and execute their complete 16-turn schedules, and
the non-agent methods execute their registered horizons without emitting stop
actions.

\subsection{Planner Output Objects}

The planner returns exactly one of the following objects. Additional top-level
fields and incomplete weight vectors are invalid.

\begin{promptbox}{Planner output: complete proposal}
\begin{promptjson}
{
  "action": "propose_weights",
  "request_full_verifier": <true or false>,
  "weights": {
    "PTV56_coverage": <0.25-4.0>,
    "PTV63_coverage": <0.25-4.0>,
    "PTV70_coverage": <0.25-4.0>,
    "Brainstem_sparing": <0.25-4.0>,
    "SpinalCord_sparing": <0.25-4.0>,
    "RightParotid_sparing": <0.25-4.0>,
    "LeftParotid_sparing": <0.25-4.0>,
    "Esophagus_sparing": <0.25-4.0>,
    "Larynx_sparing": <0.25-4.0>,
    "Mandible_sparing": <0.25-4.0>,
    "ring_falloff": <0.25-4.0>,
    "posterior_neck_sparing": <0.25-4.0>
  }
}
\end{promptjson}
\end{promptbox}

\begin{promptbox}{Planner output: stop action}
\begin{promptjson}
{
  "action": "stop",
  "request_full_verifier": false,
  "weights": null
}
\end{promptjson}

\smallskip
Stopping is valid only when \texttt{stop} appears in the turn's
\texttt{allowed\_actions}. A stop action can never request a full solve.
\end{promptbox}

\subsection{Role-Specific Prompts}

\paragraph{Evaluator planner.}
Before the planner acts, the evaluator receives the same public observation and
DVH diagram, when enabled. Its system instruction is: diagnose only from supplied
public values; never claim access to an expert reference dose; prioritize target
coverage, then critical serial or maximum-dose organs, then discretionary
mean-dose sparing; explicitly identify uncertainty and surrogate/full-solve disagreement;
and remain advisory by emitting neither weights nor the final action. The
planner receives the resulting object under \texttt{planner\_critique}.

\begin{promptbox}{Evaluator output JSON template}
\begin{promptjson}
{
  "summary": "<state diagnosis>",
  "priority_issues": [
    {"criterion": "<criterion>",
     "status": "<violated|satisfied|tradeoff|uncertain>",
     "evidence": "<public evidence>"}, ...],
  "recommended_adjustments": [
    {"objective_name": "<one of the 12 controls>",
     "direction": "<increase|decrease|hold>",
     "reason": "<publicly supported reason>"}, ...],
  "verifier_request_worth_considering": <bool>,
  "verifier_reason": "<reason>",
  "confidence": "<low|medium|high>"
}
\end{promptjson}
\end{promptbox}

\paragraph{Candidate critic.}
Except in the fixed clinical-only control of Section~\ref{supp:fixed_clinical_only}, where critic invocation follows the registered fidelity schedule, the candidate critic is called only for a planner proposal that requests a full
evaluation. It receives the public observation and the proposed action. Its system instruction is to check for avoidable target compromise,
unsupported weight--response assumptions, duplicate or negligible changes, and
whether the requested full call is likely to provide useful information. It
must use public evidence only and cannot claim access to the expert reference, emit
replacement weights, or determine which action is executed.

\begin{promptbox}{Candidate-critic input payload}
\begin{promptjson}
<PUBLIC_OBSERVATION>
  {<complete planner input JSON object>}
</PUBLIC_OBSERVATION>
<PROPOSED_ACTION>
  {<complete proposal JSON object>}
</PROPOSED_ACTION>
\end{promptjson}
\end{promptbox}

When the critic requests a revision, the planner receives its original proposal,
the advisory critique, and a statement that it may keep, revise, or
replace its weights. Exactly one revision call is permitted. The critic never
edits the proposal directly, and the planner remains responsible for the final
vector and full-request decision.

\begin{promptbox}{Candidate-critic output object}
\begin{promptjson}
{
  "verdict": "<accept|revise>",
  "issues": [
    {"issue_type": "<target_compromise|unsupported_response|duplicate_or_negligible|low_value_full_request|clinical_tradeoff>",
     "evidence": "<public evidence>",
     "severity": "<low|medium|high>"}, ...],
  "revision_guidance": "<specific advisory guidance>",
  "full_request_assessment": "<worthwhile|uncertain|low_value>",
  "confidence": "<low|medium|high>"
}
\end{promptjson}
\end{promptbox}

\subsection{Memory-View Construction}
\label{supp:memory_views}

The three memory mechanisms differ only in how the \texttt{memory\_view} field of
the planner input object is populated. All three are deterministic and are
rebuilt from scratch from the complete public trajectory before every model
decision; none relies on hidden incremental state. Given an episode trace, the
exact memory view presented at every turn is reproducible.

\paragraph{Lossless full history.}
Every prior environment step is retained in chronological order. Nothing is
dropped or summarized, including surrogate-only evaluations, full-solve
evaluations, rejected or malformed actions, duplicate proposals, and stop
actions. No length cap or truncation is applied, so the 16-turn horizon exposes
at most 16 prior steps.

\paragraph{Criterion-response contrast.}
The reported configuration uses \texttt{recent\_steps}~$=2$. The view is the
union of the two most recent environment steps, regardless of acceptance or
fidelity; the current best-surrogate incumbent, if one exists; the current best
successful-full-solve incumbent, if one exists; the most recent successful full
solve; and best and worst full-solve examples for the active criterion. Exactly
one best-surrogate and one best-full incumbent pointer are carried, and the union
removes repeated step indices while combining their selection reasons.

The active criterion is determined from the most recent successful full solve.
Among its strictly positive clinical-criterion violations, the criterion with the
largest violation magnitude is selected; an exact magnitude tie is broken by the
lexicographically larger criterion name. If every violation is zero, no contrast
pair is added. The best and worst examples are then chosen from all successful
full-solve steps containing that criterion: best is the smallest violation and
worst the largest, with exact ties resolved in favor of the earlier step.
Surrogate-only turns are not eligible for these criterion-specific roles, though
they may still enter the view through recency or as the best-surrogate
incumbent. Duplicate proposals remain distinct history entries; when duplicate
full-solve entries carry identical criterion values, the earlier entry wins both
exact-value tie breaks unless the later one is retained through recency or
another incumbent role.

\paragraph{Pareto-tradeoff.}
This mechanism augments lossless full history rather than replacing or
truncating it, so no separate recency window is used and the entire history
remains visible alongside the archive. It adds verified response records for
full-request steps, containing the weights, the weight changes from the
preceding accepted proposal, the public surrogate and full metrics, the
criterion violations, and the changes from the preceding full result; and a
Pareto archive over successful full solves only.

For each successful full solve the lower-is-better Pareto vector contains the
mean clinical-criterion violation, falling back to the objective where that
value is unavailable, together with every available individual clinical
violation clipped as $\max(0,v_i)$. Dominance is evaluated over the objective
keys shared by all eligible candidates,
%
\begin{equation}
a \prec b \iff a_k \leq b_k\ \ \forall k
\quad\text{and}\quad a_k < b_k\ \text{for at least one } k.
\end{equation}
%
Failed and timed-out full solves cannot enter the frontier, and surrogate-only
turns cannot enter it although they remain visible in the full history. There is
no archive-size cap or truncation rule, and frontier order follows original step
order. Equal objective vectors do not dominate one another, since strict
improvement on at least one objective is required, so both are retained, and
exact duplicate candidates remain separate history and archive entries when
nondominated. The frontier therefore holds at most three successful full-solve
entries in the primary condition and at most sixteen in the 16-solve condition.

The fixed clinical-only control uses the contrast structure with a scalar
substitution, described in Section~\ref{supp:fixed_clinical_only}.

\subsection{Fixed Clinical-Only Control}
\label{supp:fixed_clinical_only}

The fixed clinical-only control uses criterion-response contrast memory with the candidate-critic role, as in the main agent conditions. It preserves the common system instruction,
public case description, clinical protocol, meanings and bounds of the 12
controls, scalar clinical outcomes, surrogate-verifier uncertainty, and public
history. It removes per-criterion feedback, numerical DVH metrics, and the
rendered DVH diagram. After a full solve it receives no optimized-plan summaries
at all: the returned feedback is the scalar $\Delta J_{\mathrm{clin}}$ together with the
solve status and cost, matching the outcome feedback available to the non-agent
methods. Criterion-response contrast memory therefore operates in scalar form in
this control. Contrasting best- and worst-response examples are selected among
successful full solves by the mean clinical-criterion violation rather than by a
dominant individual criterion: best is the lowest violation and worst the
highest, with exact ties resolved in favor of the earlier step. No active
criterion is computed, and the retained examples carry weights and scalar
outcomes only. No criterion
identity or per-criterion value enters memory, so the mechanism becomes a
scalar best/worst contrast over prior turns. Routing is fixed rather than chosen
by the model: turns 1--13 are surrogate evaluations and turns 14--16 are full
solves. The turn payload therefore adds the following fields, and stopping is
disabled.

\begin{promptbox}{Fixed-schedule planner rules}
\begin{promptjson}
{
  "turn_number_one_indexed": <1-16>,
  "horizon_turns": 16,
  "full_verifier_turns_one_indexed": [14,15,16],
  "this_turn_fidelity": "<cheap_only|full>",
  "contract": {
    "routing_is_fixed_by_experiment": true,
    "planner_must_propose_complete_weights_every_turn": true,
    "planner_must_not_stop_early": true,
    "request_full_verifier_must_equal_schedule": <false|true>,
    "candidate_critic_reviews_weights_not_routing": true
  }
}
\end{promptjson}
\end{promptbox}

This control contains a known prompt--environment inconsistency. The common
agent-choice instruction reproduced in
Section~\ref{supp:prompt_overview_common} tells the planner that there is no
external router and that the environment does not force or rewrite an action.
That statement does not hold in this condition: the planner receives the
instruction unchanged while the environment overwrites its routing decisions.
Where the two conflict, the turn-specific schedule fields determine what is
executed. After a structurally valid
action is parsed, the environment preserves the planner's proposed weight vector
but overwrites its fidelity request according to the registered schedule,
setting \texttt{request\_full\_verifier} to false on turns 1--13 and true on
turns 14--16, and setting \texttt{stop} to false on every turn. The candidate critic is invoked on
the three full-solve turns and not on surrogate turns. A fidelity
mismatch is ignored rather than rejected or retried, and triggers no additional
attempt; only ordinary structured-output errors follow the rejection path of
Section~\ref{supp:prompt_overview_validation}. The
\texttt{request\_full\_verifier\_must\_equal\_schedule} field is named
misleadingly in the frozen artifact: it carries the required fidelity value for
the current turn, false on surrogate turns and true on full-solve turns, rather
than a Boolean enabling equality validation. It duplicates \texttt{this\_turn\_fidelity}.

The planner is therefore told it controls routing when it does not. Any effect
this has on its proposals cannot be separated from the effects the condition is
meant to isolate, so the condition controls feedback content and the scheduled
number of full solves rather than routing or the prompt itself. Matched scalar
feedback also does not imply matched adaptation: the language controller remains sequentially adaptive across the three terminal full solves, generating each new candidate after seeing the previous full-solve outcome, whereas the non-agent terminal candidates are frozen before any of those solves.

\subsection{Validation, Retries, and Model Settings}
\label{supp:prompt_overview_validation}

The parser requires exactly \texttt{action},
\texttt{request\_full\_verifier}, and \texttt{weights}; extra properties are
forbidden. It rejects malformed JSON, unknown or missing controls, non-finite
values, weights outside $[0.25,4.0]$, illegal stop/full combinations, and
requests exceeding the remaining budget. Evaluator and candidate-critic
objects are validated with the same exact-field policy, enumerated categorical
values, and at most five issues or adjustments. Semantic response repair is
disabled.

Transport recovery remains inside one logical language decision and therefore
does not consume another environment turn. GPT planner/evaluator/critic calls
permit up to seven attempts for transient transport failures; Qwen permits up
to three. Claude uses native structured output without response repair; no transport retry was recorded on the Claude route. The
three backbones use their default reasoning configurations. Every recorded trace contains the public
input object, attached optimized-plan DVH when enabled, raw structured response,
validated action, public outcome, and retry count.
