# Supplementary material for: RadOncGym: An Agent-Based Framework for Radiotherapy Dose-Mimicking Optimization
Source: arXiv:2611.33821 source file (2026-11-25)
Supplement: Supplementary file 7 [file reproducibility.tex]

\section{Reproducibility Details}
\label{supp:reproducibility}

This section provides the model, solver, runtime, verifier-development, and release details referenced by the main paper.

\subsection{Terminology}
We use the terms of the main paper throughout the supplement: the \emph{surrogate verifier} is the learned scorer; a \emph{full solve} is a Gurobi planning solve; budgets are counted in \emph{full-solve attempts}, which include timeouts and exact-cache replays, while reported outcome counts are \emph{successful full solves}; and the \emph{non-agent methods} are Sobol, CMA-ES, Exact-GP LogEI, and SAAS-BO. Information described as \emph{public} is visible to the agent during optimization; the expert reference dose and the DVH and dose scores are not. The agent-facing JSON interface reproduced in Section~\ref{supp:prompt_interface} uses the implementation names \texttt{cheap} and \texttt{full} for the two fidelities and is shown as the model receives it; the instruction also calls the full solve the \emph{physics verifier} or the \emph{expensive verifier}.

Improvement is reported as
$\Delta J_{\mathrm{clin}} = J_{\mathrm{clin}}(d_1) - J_{\mathrm{clin}}(d_w)$, so that
positive values indicate improvement over the all-ones initialization. The planner uses lower-is-better objectives. Criterion violations and plan objective values remain lower-is-better
quantities throughout.

\subsection{Models and Seeds}
All reported planner and non-agent optimizer campaigns use seed 23 and ran in August 2026. Seed 23 controls the environment, optimizer, and other local random number generators. The language-model routes expose no sampling seed and use provider defaults, so seed 23 does not make provider model outputs deterministically replayable.
The planner identifiers are \texttt{gpt-5.6-sol} through Codex CLI 0.147.0, \texttt{claude-sonnet-5} through Claude Code CLI 2.1.233, and \texttt{qwen3.6-27b} through the DashScope OpenAI-compatible Beijing endpoint with OpenAI Python SDK 2.54.0. Each route uses its default reasoning setting: medium for GPT and Claude, and thinking enabled with a 4096-token budget for Qwen. None of the three routes exposes or sends a temperature, top-$p$, or output-token setting, so all use provider defaults. GPT and Claude were accessed through subscription execution routes rather than metered APIs, keeping a campaign of this size within an academic research budget; the model identifier, prompt, and structured-output schema supplied by our runner are the same on either route. All planner actions use structured JSON-Schema output.
In the cross-model comparison, all three backbones use criterion-response contrast memory with the candidate-critic role and support image input; the memory--role comparison varies both factors for GPT-5.6 Sol. Numerical DVH metrics and a rendered DVH diagram for the optimized plan are provided only after a successful full solve, and are unavailable on surrogate-only turns. The nine memory/role configurations and the architecture used for the cross-model comparison were fixed in advance of the final-cohort results.

\subsection{Agent Textual Interface}
The common planner system instruction is fixed text and is reproduced in full
in Section~\ref{supp:prompt_overview_common}. The surrounding observation is
constructed programmatically for each turn, so no single stored prompt string
exists for a complete turn. The common observation fields, the per-criterion and DVH feedback added after a full solve, the fixed clinical-only omissions, and the structured action interface are documented in Section~\ref{supp:agent_observation}.

\subsection{Planning Backend and Optimizer Settings}
The planning backend is Gurobi 11.0.3 through OR-Tools 9.10.4067 (\texttt{GUROBI\_LP}), using the full-resolution \texttt{absolute\_mean} formulation with \texttt{Method=2}, \texttt{Crossover=0}, \texttt{BarConvTol=}$10^{-5}$, \texttt{BarHomogeneous=1}, four solver threads, and a 1800-s time limit per full solve. A local compatibility patch alters solver selection and status handling only and does not change the linear program.
Table~\ref{tab:supp_optimizer_settings} lists the non-agent optimizer settings. Sobol uses the common all-ones anchor followed by the seeded Sobol sequence. The anchor is the precomputed all-ones plan and does not consume one of the 13 surrogate-screening turns.

\begin{table}[!t]
\centering
\small
\setlength{\tabcolsep}{4pt}
\begin{tabular*}{\columnwidth}{@{\extracolsep{\fill}}lP{0.66\columnwidth}@{}}
\toprule
Method & Settings \\
\midrule
CMA-ES & population 11, $\sigma=0.45$ \\
\addlinespace[2pt]
Exact-GP LogEI & initial design 4; 256 raw samples; 16 restarts; $\le$200 GP-fitting iterations \\
\addlinespace[2pt]
SAAS-BO & initial design 4; 256 raw samples; 16 restarts; 128 NUTS warmup steps; 64 NUTS samples; thinning 4; max tree depth 6; 256 acquisition Monte Carlo samples \\
\bottomrule
\end{tabular*}
\caption{\textbf{Non-agent optimizer settings.} The same configuration is used at both solve budgets.}
\label{tab:supp_optimizer_settings}
\end{table}


Experiments used Python 3.10.20; the verifier artifact was serialized with scikit-learn 1.7.2, CMA-ES uses \texttt{cma} 4.4.4, and Exact-GP LogEI and SAAS-BO use BoTorch 0.16.1, GPyTorch 1.15.2, and PyTorch 2.12.0.
In the three-solve non-agent track, 13 surrogate clinical-screening actions precede three full solves. Sobol, CMA-ES, Exact-GP LogEI, and SAAS-BO retain their standard scalar interfaces and do not jointly model surrogate-verifier and Gurobi outcomes or select fidelity online; an interleaved schedule would require a separate adaptive multi-fidelity implementation.

\subsection{Runtime Accounting}
Experiments ran on an institutional Slurm cluster.
Reported solver cost is elapsed wall time around each full solve, summed per context; Slurm queue time and provider-gate waiting are excluded.
Non-agent method runtime adds optimizer/update and runner overhead, while GPT and Claude runtime uses low-contention, capacity-normalized call latency to avoid attributing rare provider stalls to algorithmic time. We recorded no provider-gate waiting on the Qwen route, so its measured call time is taken as the algorithmic time.
Exact-cache replays retain the logical cost of the original solve and are not counted as zero-cost evaluations.

For method $m$ and patient--prediction context $c$, normalized active time is
defined as
\begin{equation}
T^{\mathrm{active}}_{m,c}
=
\sum_{s\in\mathcal{S}_{m,c}} t^{\mathrm{solve}}_{c,s}
+ t^{\mathrm{runner}}_{m,c}
+ \sum_{q\in\mathcal{Q}_{m,c}} \bar{\tau}_{g(q)},
\label{eq:supp_active_time}
\end{equation}
where $\mathcal{S}_{m,c}$ is the set of charged full solves,
$t^{\mathrm{runner}}_{m,c}$ includes optimizer updates and orchestration, and
$\mathcal{Q}_{m,c}$ is the set of language-model calls. For GPT and Claude,
the normalized latency assigned to call group $g$ is
\begin{equation}
\bar{\tau}_{g}
=
\frac{1}{|\mathcal{R}_{g}|}
\sum_{q\in\mathcal{R}_{g}}
\left(t^{\mathrm{wall}}_{q}-t^{\mathrm{gate}}_{q}\right),
\label{eq:supp_call_time}
\end{equation}
with $\mathcal{R}_{g}$ the low-contention reference calls in the same call-type
and turn-position group. The non-agent methods have
$\mathcal{Q}_{m,c}=\varnothing$. The reported minutes per context are
\begin{equation}
\overline{T}_{m}
=
\frac{1}{|\mathcal{C}|}
\sum_{c\in\mathcal{C}} T^{\mathrm{active}}_{m,c},
\qquad |\mathcal{C}|=600,
\label{eq:supp_mean_time}
\end{equation}
after converting seconds to minutes. For Qwen, Eq.~\eqref{eq:supp_call_time}
reduces to the measured call time.

\subsection{Campaign Accounting}
Both GPT-5.6 Sol campaigns cover the same 60 patients and 600 patient--prediction contexts. In the 16-solve campaign, mean solver time is 124.088 min/context (median 89.11) and normalized model time is 12.240 min/context, giving a normalized full-method runtime of 136.328 min/context. For the primary three-solve campaign, the
corresponding values are 23.376 min/context of Gurobi solver time and 4.074
min/context of capacity-normalized model time. These rounded components sum,
using their unrounded values, to the 27.449 min/context reported in the main
comparison table. Model time
covers planner, candidate-critic, and planner-revision calls. No
numerical-optimizer update time applies to a language condition, and runner
overhead was not measured or charged separately for it. Table~\ref{tab:supp_campaign} reports model invocations, full-solve outcomes, and audit results for both conditions.

\begin{table}[!t]
\centering
\footnotesize
\setlength{\tabcolsep}{4pt}
\begin{tabular*}{\columnwidth}{@{\extracolsep{\fill}}P{0.46\columnwidth}rr@{}}
\toprule
Quantity & Three-solve & 16-solve \\
\midrule
\multicolumn{3}{@{}l}{\textbf{Model invocations}} \\
Planner & 5,953 & 9,600 \\
Candidate critic & 2,016 & 9,600 \\
Planner revision & 358 & 6,225 \\
Total & 8,327 & 25,425 \\
Per context & 13.878 & 42.375 \\
\addlinespace[2pt]
\multicolumn{3}{@{}l}{\textbf{Full-solve outcomes}} \\
Requests & 1,765 & 9,600 \\
Successful solves & 1,732 & 9,379 \\
Timeouts & 33 & 221 \\
Other solver failures & 0 & 0 \\
\addlinespace[2pt]
\multicolumn{3}{@{}l}{\textbf{Context-level outcomes}} \\
With a timeout but a valid plan & 16 & 15 \\
With no successful solve & 5 & 9 \\
Invalid executed actions & 0 & 0 \\
Post-hoc audits passed & 600/600 & 600/600 \\
\bottomrule
\end{tabular*}
\caption{\textbf{Model invocations, full-solve outcomes, and audits for the two
GPT-5.6 Sol campaigns.} Stopping is disabled in the 16-solve condition, so its
planner and candidate-critic counts are exactly 16 per context. In the
three-solve condition the candidate critic is invoked on proposed escalations
rather than on every turn, and its count exceeds the 1,765 executed requests
because the critic sometimes intercepted a proposed escalation that the planner
then revised to a surrogate-only action. Timeout is the only observed solver
failure, so contexts with no successful solve are exactly those whose every
attempt timed out; each falls back to the all-ones plan.}
\label{tab:supp_campaign}
\end{table}

A call is low-contention if it lasts at most 60~s after recorded provider-gate waiting is subtracted; 16,002 such calls set the group latencies in Eq.~\eqref{eq:supp_call_time}. This is a standardized algorithmic-time estimate rather than provider-side GPU time. Recorded episode wall time is 128.21 min/context (median 92.19); it excludes Slurm queueing and includes agent and provider-gate waiting. The normalized full-method runtime exceeds it because exact-cache replays are charged the logical cost of the original solve rather than their elapsed time. A replay is a repeat request for a weight vector already solved in that context, and it returns the stored plan without running a new solve. Charged solver time is therefore larger than elapsed solver time. The cost--performance analysis uses the normalized full-method runtimes reported in the main comparison table; for Exact-GP LogEI, SAAS-BO, CMA-ES, and Sobol at budget 16, these are 112.062, 122.680, 109.913, and 110.463 min/context, respectively. In the 16-solve condition, 576 contexts solve all 16 attempts successfully, 15 record at least one timeout while still yielding a valid selected plan, and 9 time out on every attempt and fall back to the all-ones plan.

The final normalized runtime is 21.25 min/context for fixed clinical-only GPT-5.6 Sol, 21.65 min/context for Adaptive LogEI, and 37.55 min/context for the 64-turn extended Exact-GP LogEI control. These totals use the same active-time convention as the main comparison.

\subsection{Verifier Development}
Surrogate-verifier development records 6,400 full-solve attempts over the 40-patient training and validation cohort, of which 342 time out. The fitting and validation sets contain the remaining 4,618 and 1,440 rows.

\subsection{Release and Licensing}
RadOncGym code and configurations are available under the MIT license.
The release preserves the upstream OpenKBP-Opt MIT software license, README, and citation, while directing users to the official upstream data downloads instead of mirroring CT volumes, masks, reference doses, submitted predictions, or official plan archives until data-specific redistribution permission is confirmed.

\paragraph{Released package.}
The public package is a minimal reference implementation: the environment and evaluation code, prompt and schema construction code, controller definitions, the experiment configurations for the reported conditions, and the frozen surrogate-verifier artifact together with its ordered feature schema. Reproducing Gurobi-based planning requires a separately obtained commercial or academic Gurobi license.
