# Supplementary material for: RadOncGym: An Agent-Based Framework for Radiotherapy Dose-Mimicking Optimization
Source: arXiv:2611.33821 source file (2026-11-25)
Supplement: Supplementary file 8 [file statistical_uncertainty.tex]

\section{Patient-Clustered Uncertainty}
\label{supp:uncertainty}

We treat the 60 patients, rather than the 600 patient--prediction contexts, as the independent units. Confidence intervals use 10,000 bootstrap replicates (seed 20260824), resampling patients with replacement and retaining all ten prediction contexts for each sampled patient. Reported intervals are percentile intervals: the 2.5th and 97.5th percentiles of the replicate distribution.

\begin{table*}[!t]
\centering
\small
\setlength{\tabcolsep}{4pt}
\renewcommand{\arraystretch}{1.08}
\begin{tabular*}{\textwidth}{@{\extracolsep{\fill}}lccc@{}}
\toprule
\multicolumn{4}{l}{\textbf{(a) Marginal improvement over the context-matched all-ones plan}} \\
\addlinespace[2pt]
Method & Clinical criterion, Gy & DVH score, Gy & Dose score, Gy \\
& Mean [95\% CI] & Mean [95\% CI] & Mean [95\% CI] \\
\midrule
Sobol-3          & $0.084\ [0.053,0.120]$   & $0.087\ [0.021,0.159]$    & $0.008\ [-0.037,0.056]$ \\
CMA-ES-3         & $0.083\ [0.053,0.116]$   & $0.259\ [0.186,0.333]$    & $0.037\ [0.003,0.073]$ \\
Exact-GP-3       & $0.155\ [0.114,0.197]$   & $0.247\ [0.175,0.335]$    & $0.088\ [0.041,0.141]$ \\
SAAS-BO-3        & $0.228\ [0.176,0.283]$   & $-0.075\ [-0.174,0.042]$ & $0.096\ [0.034,0.162]$ \\
\addlinespace[2pt]
Adaptive LogEI   & $0.236\ [0.167,0.308]$   & $0.070\ [-0.022,0.176]$  & $0.039\ [-0.025,0.097]$ \\
\addlinespace[2pt]
\textbf{GPT-5.6 Sol} & $\mathbf{0.613\ [0.490,0.729]}$ & $\mathbf{0.599\ [0.484,0.718]}$ & $\mathbf{0.220\ [0.126,0.322]}$ \\
Claude Sonnet 5  & $0.486\ [0.385,0.586]$   & $0.342\ [0.248,0.440]$    & $0.182\ [0.107,0.260]$ \\
Qwen3.6-27B      & $0.405\ [0.322,0.489]$   & $0.175\ [0.085,0.266]$    & $0.151\ [0.084,0.220]$ \\
\midrule
\multicolumn{4}{l}{\textbf{(b) Paired difference: GPT-5.6 Sol minus comparator}} \\
\addlinespace[2pt]
Comparator & Clinical criterion, Gy & DVH score, Gy & Dose score, Gy \\
& 95\% CI & 95\% CI & 95\% CI \\
\midrule
Sobol-3          & $[0.404,0.644]$ & $[0.395,0.627]$ & $[0.120,0.316]$ \\
CMA-ES-3         & $[0.413,0.640]$ & $[0.221,0.466]$ & $[0.098,0.274]$ \\
Exact-GP-3       & $[0.356,0.552]$ & $[0.231,0.467]$ & $[0.051,0.228]$ \\
SAAS-BO-3        & $[0.295,0.466]$ & $[0.522,0.817]$ & $[0.047,0.222]$ \\
\addlinespace[2pt]
Adaptive LogEI   & $[0.311,0.434]$ & $[0.408,0.644]$ & $[0.111,0.259]$ \\
\addlinespace[2pt]
Claude Sonnet 5  & $[0.093,0.156]$ & $[0.197,0.319]$ & $[0.004,0.077]$ \\
Qwen3.6-27B      & $[0.153,0.257]$ & $[0.344,0.503]$ & $[0.023,0.124]$ \\
\bottomrule
\end{tabular*}
\caption{\textbf{Patient-clustered uncertainty for the matched three-solve comparison.} Panel (a) reports the mean improvement and marginal 95\% confidence interval relative to the all-ones plan; positive values indicate improvement. Panel (b) reports paired 95\% confidence intervals for the improvement difference between GPT-5.6 Sol and each comparator; positive values favor GPT-5.6 Sol. Pairing is by patient and prediction set.}
\label{tab:supp_uncertainty}
\end{table*}

Every paired interval in Table~\ref{tab:supp_uncertainty}(b) lies above zero.

\subsection{Memory and Role-Structure Comparison}

Table~\ref{tab:supp_memory_role_paired} pairs each of the remaining eight
memory--role configurations against criterion-response contrast memory with the
candidate critic, the configuration used for the cross-model comparison in the
main paper. Positive values favor that reference. Point estimates are the
differences of the means in the main-paper memory--role table, and the intervals
use the resampling procedure described above.

Under criterion-response contrast memory, the candidate-critic versus
direct-planner intervals contain zero on all three endpoints, with mean
differences of $+0.003$, $-0.007$, and $+0.000$~Gy. Lossless full history
with the direct planner likewise has intervals containing zero on all three.
Across the eight reference comparisons, 11 of the 24 endpoint-specific
intervals exclude zero. These are pointwise intervals, unadjusted for
multiplicity.

Other comparisons show endpoint-specific differences. The evaluator-planner role has lower
clinical-criterion and DVH improvements than the reference under all three
memory mechanisms, by 0.072--0.091~Gy and 0.095--0.138~Gy respectively, with
intervals excluding zero in every case. Pareto-tradeoff memory has lower
clinical-criterion improvement with both the direct planner and the candidate
critic, and with the candidate critic also lower DVH improvement. Lossless full history
with the candidate critic has lower clinical-criterion improvement by 0.010~Gy
but higher dose improvement by 0.013~Gy.

Seven of the eight dose-score intervals contain zero; the remaining interval
favors lossless full history with the candidate critic. No comparator is
separated from the reference on all three endpoints simultaneously.


\begin{table*}[!t]
\centering
\small
\setlength{\tabcolsep}{1pt}
\renewcommand{\arraystretch}{1.08}
\begin{tabular*}{\textwidth}{@{\extracolsep{\fill}}llccc@{}}
\toprule
\multicolumn{5}{@{}l}{\textbf{Paired difference: criterion-response contrast with candidate critic minus comparator}} \\
\addlinespace[2pt]
Memory & Role & Clinical criterion, Gy & DVH score, Gy & Dose score, Gy \\
& & Mean [95\% CI] & Mean [95\% CI] & Mean [95\% CI] \\
\midrule
Lossless full history & Direct planner & $+0.005\ [-0.006,+0.017]$ & $-0.013\ [-0.036,+0.011]$ & $-0.006\ [-0.015,+0.005]$ \\
\textbf{Criterion-response contrast} & \textbf{Direct planner} & $\mathbf{+0.003\ [-0.005,+0.011]}$ & $\mathbf{-0.007\ [-0.035,+0.020]}$ & $\mathbf{+0.000\ [-0.010,+0.010]}$ \\
Pareto-tradeoff & Direct planner & $+0.021\ [+0.010,+0.033]$ & $+0.014\ [-0.011,+0.039]$ & $+0.005\ [-0.005,+0.016]$ \\
\addlinespace[2pt]
Lossless full history & Candidate critic & $+0.010\ [+0.001,+0.019]$ & $+0.004\ [-0.019,+0.026]$ & $-0.013\ [-0.024,-0.002]$ \\
Pareto-tradeoff & Candidate critic & $+0.028\ [+0.014,+0.043]$ & $+0.027\ [+0.005,+0.049]$ & $-0.003\ [-0.015,+0.011]$ \\
\addlinespace[2pt]
Lossless full history & Evaluator planner & $+0.072\ [+0.051,+0.095]$ & $+0.095\ [+0.060,+0.130]$ & $+0.004\ [-0.017,+0.026]$ \\
Criterion-response contrast & Evaluator planner & $+0.080\ [+0.057,+0.105]$ & $+0.105\ [+0.065,+0.145]$ & $+0.010\ [-0.012,+0.033]$ \\
Pareto-tradeoff & Evaluator planner & $+0.091\ [+0.067,+0.117]$ & $+0.138\ [+0.097,+0.179]$ & $+0.011\ [-0.009,+0.033]$ \\
\bottomrule
\end{tabular*}
\caption{\textbf{Paired patient-clustered differences among the nine GPT-5.6 Sol memory--role configurations.} Each row compares the reference configuration, criterion-response contrast memory with the candidate critic, against one of the other eight. Positive values favor the reference. Pairing is by patient and prediction set. The bold row is the comparison between the two role structures under the memory mechanism used elsewhere in the paper; all three of its intervals contain zero.}
\label{tab:supp_memory_role_paired}
\end{table*}
