# Supplementary material for: RadOncGym: An Agent-Based Framework for Radiotherapy Dose-Mimicking Optimization
Source: arXiv:2611.33821 source file (2026-11-25)
Supplement: Supplementary file 9 [file surrogate_verifier.tex]

\section{Surrogate-Verifier Details}
\label{supp:verifier_details}

The frozen surrogate verifier is a 24-member ensemble of histogram-based gradient-boosting regressors. Its input has 309 values: the candidate's 12 objective weights followed by the 297-value public context vector described in Section~\ref{supp:agent_observation}. It predicts only the clinical-criterion improvement relative to the context-matched all-ones plan and an uncertainty estimate; it never predicts individual violations, DVH score, or dose score.

\subsection{Ordered Feature Schema}

Table~\ref{tab:supp_verifier_schema} enumerates all 309 positions. Repeated blocks follow the displayed object and field orders, so every feature and its position is specified.

\begin{table*}[!t]
\centering
\small
\setlength{\tabcolsep}{4pt}
\renewcommand{\arraystretch}{1.08}
\begin{tabular}{@{}P{0.085\textwidth}P{0.075\textwidth}P{0.335\textwidth}P{0.455\textwidth}@{}}
\toprule
Zero-based index & Count & Ordered objects & Ordered fields \\
\midrule
0--11 & 12 & Objective controls & The 12 controls in Table~\ref{tab:supp_controls}, in table order \\
12--17 & 6 & Global anatomy & voxel spacing $x,y,z$; voxel volume; possible-dose voxel count; possible-dose volume \\
18--25 & 8 & CT within stored grid & min, mean, max, p01, p05, p50, p95, p99 \\
26--33 & 8 & Prediction within possible-dose mask & min, mean, max, p01, p05, p50, p95, p99 \\
34--203 & $10\times17$ & Brainstem, SpinalCord, RightParotid, LeftParotid, Esophagus, Larynx, Mandible, PTV56, PTV63, PTV70 & present; voxel count; volume; centroid fraction $x,y,z$; bounding-box extent $x,y,z$; predicted-dose min, mean, max, p01, p05, p50, p95, p99 \\
204--287 & $7\times3\times4$ & Brainstem, SpinalCord, RightParotid, LeftParotid, Esophagus, Larynx, Mandible, each crossed with PTV56, PTV63, PTV70 & intersection volume; fraction of OAR; fraction of PTV; Dice coefficient \\
288--308 & 21 & Prediction identity & one-hot indicators \texttt{set\_1}, $\ldots$, \texttt{set\_21} \\
\bottomrule
\end{tabular}
\caption{\textbf{Ordered 309-feature schema for the surrogate verifier.} Within each repeated block, the object order is outermost and the field order is innermost. The final evaluation uses prediction sets 1--10, but the frozen schema retains all 21 released identifiers.}
\label{tab:supp_verifier_schema}
\end{table*}

Missing structures retain their fixed positions with \texttt{present}$=0$ and zero-filled numeric fields. Centroids are normalized by grid extent, bounding boxes are inclusive voxel extents multiplied by voxel spacing, and empty-region overlap statistics are zero. No feature contains the expert reference dose or any reference-derived endpoint.

\subsection{Development Split and Uncertainty Estimate}

The verifier-development cohort uses 30 training patients and 10 validation patients, all disjoint from the 60 evaluation patients. It contains 4,618 fitting rows and 1,440 validation rows.

The cohort is the full 100-patient OpenKBP-Opt set, \texttt{pt\_241} through
\texttt{pt\_340}, so the three groups partition it exactly and patient
disjointness holds by construction. The split was drawn at random, was frozen
before any final-cohort result was examined, and is included with the released
code. The 30 training patients are \texttt{pt\_241, pt\_242, pt\_248, pt\_249, pt\_252, pt\_254, pt\_255, pt\_256, pt\_270, pt\_272, pt\_273, pt\_276, pt\_277, pt\_282, pt\_284, pt\_287, pt\_290, pt\_295, pt\_297, pt\_301, pt\_306, pt\_310, pt\_317, pt\_320, pt\_321, pt\_323, pt\_328, pt\_335, pt\_338, pt\_339}. The 10 validation
patients are \texttt{pt\_250, pt\_260, pt\_262, pt\_268, pt\_283, pt\_294, pt\_307, pt\_311, pt\_313, pt\_319}. The 60 evaluation patients are the remaining
members of the cohort. Verifier development uses the same ten prediction sets,
1--10, applied to the 40 development patients, giving 400 development contexts
against the 600 evaluation contexts. The partition is by patient, so no
evaluation patient contributes a fitting or validation row and no evaluation
context is solved during development. These are the 10 held-out patients used in the verifier figure in the main paper. They are held out from regressor fitting and are also the cohort on which the ensemble was selected, so the diagnostics below are validation diagnostics; the 60 evaluation patients are the patient-disjoint cohort used for the planning-method comparisons. We evaluated all 72 hyperparameter configurations, spanning loss, learning rate, leaf count, minimum leaf samples, and $L_2$ regularization, on the verifier-validation cohort using seed 17, and screened them jointly on context-delta mean absolute error, within-context Spearman correlation, pairwise preference accuracy, top-1 recovery, top-3 retention, and selection regret. We retained configurations 7, 15, 31, 43, 62, and 67 as the multi-metric stability set, listed in Table~\ref{tab:supp_hgbr}, refit each using seeds 17, 29, 43, and 71, and averaged all 24 resulting models. The resulting ensemble is included in the release, so its prediction for any weight vector and context is exactly reproducible. The verifier is frozen before every evaluation campaign and does not update from agent trajectories.

\begin{table}[!t]
\centering
\small
\setlength{\tabcolsep}{4pt}
\begin{tabular*}{\columnwidth}{@{\extracolsep{\fill}}lcccc@{}}
\toprule
Loss & Learning rate & Max leaves & Min leaf & $L_2$ \\
\midrule
Squared error  & 0.03 & 31 & 30 & 3.0 \\
Squared error  & 0.05 & 15 & 30 & 3.0 \\
Squared error  & 0.10 & 31 & 30 & 3.0 \\
Absolute error & 0.03 & 31 & 30 & 3.0 \\
Absolute error & 0.10 & 15 & 30 & 0.3 \\
Absolute error & 0.10 & 31 & 30 & 3.0 \\
\bottomrule
\end{tabular*}
\caption{\textbf{The six gradient-boosting configurations in the frozen ensemble.} All use \texttt{max\_iter}~=~800 with early stopping (\texttt{validation\_fraction}~=~0.15, \texttt{n\_iter\_no\_change}~=~50) under scikit-learn 1.7.2, and each is fitted at four seeds, giving 24 members.}
\label{tab:supp_hgbr}
\end{table}

Each regressor is trained on the internal target $y(w)=J_{\mathrm{clin}}(d_w)-J_{\mathrm{clin}}(d_1)$, rather than on absolute clinical-criterion violation. This is a lower-is-better training target. Each member is scored at the candidate weights and at the all-ones weights, and its anchored prediction is the difference between the two, which forces an exact zero prediction at the all-ones anchor and removes residual context offset. The ensemble prediction is the arithmetic mean of the 24 anchored predictions. For reporting, that mean is negated to express $\Delta J_{\mathrm{clin}} = J_{\mathrm{clin}}(d_1) - J_{\mathrm{clin}}(d_w)$, for which positive values indicate predicted improvement. All reported verifier diagnostics and figures use this convention. Both axes of the verifier figure in the main paper plot $\Delta J_{\mathrm{clin}}$ in this orientation, so a positive coordinate on either axis is an improvement over the all-ones plan. The uncertainty reported with each prediction is $\sqrt{\sigma^2 + q_{90}^2}$, where $\sigma$ is the population standard deviation of the 24 anchored predictions and $q_{90} = 0.4922$~Gy is the 90th percentile of the absolute residuals of the ensemble prediction over the 1,440 validation rows. It is a percentile of absolute residuals, not a residual standard deviation or a root-mean-square error.

\subsection{Static and Adaptive-Query Evaluation}

Table~\ref{tab:supp_verifier_eval} evaluates the verifier on two candidate
populations. Static validation uses the offline candidates from the
development cohort, whereas the adaptive queries are the full-solve
requests issued by the representative GPT-5.6 Sol campaign with
criterion-response contrast memory and the candidate-critic role, so they follow
the distribution the verifier actually encounters inside the loop. Mean absolute error rises from 0.216 to
0.358~Gy under that shift and is largest during turns 5--8, while agreement
with the full solve on whether a candidate improves over the all-ones
initialization remains 81.6\%. The validation cohort contains ten patients, of which nine contribute solved
target rows to the model-selection diagnostics: one patient times out on every
candidate in all ten of its prediction contexts, removing 160 rows and
contributing none. The static diagnostics are therefore computed over
the remaining nine patients, which give 90 contexts with a complete set of 16
candidates each and the 1,440 solved surrogate--full pairs counted in the table.
Those 16 candidates include the all-ones anchor, so 90 of those rows contribute
a zero target and a zero anchored prediction; mean absolute error and every
within-context ranking diagnostic use the complete pool. Preference accuracy is the
fraction of non-tied candidate pairs within a context on which the verifier and
the full solve agree about which candidate has the larger
$\Delta J_{\mathrm{clin}}$, that is, the greater improvement over the all-ones
initialization. Top-3 retained is the fraction of contexts in which the true
best candidate falls within the verifier's three highest-ranked candidates.
Selected regret is the full-solve $\Delta J_{\mathrm{clin}}$ of the oracle-best
candidate minus that of the candidate the verifier ranks first, averaged over
contexts; zero means the verifier selected the true best.

\begin{table}[!t]
\centering
\footnotesize
\setlength{\tabcolsep}{2.5pt}
\renewcommand{\arraystretch}{1.04}
\begin{tabular*}{\columnwidth}{@{\extracolsep{\fill}}lrlr@{}}
\toprule
\multicolumn{2}{c}{\textbf{Static validation}} &
\multicolumn{2}{c}{\textbf{Adaptive queries}} \\
\cmidrule(r){1-2}\cmidrule(l){3-4}
Diagnostic & Value & Diagnostic & Value \\
\midrule
Solved pairs & 1,440 & Solved pairs & 1,732 \\
MAE (Gy) & 0.216 & MAE (Gy) & 0.358 \\
Mean Spearman & 0.705 & RMSE (Gy) & 0.492 \\
Pref. accuracy & 0.780 & Mean Spearman & 0.571 \\
Top-3 retained & 58.9\% & Sign agreement & 81.6\% \\
Selected regret (Gy) & 0.104 & Timeouts & 33 \\
\midrule
\multicolumn{4}{c}{\textbf{Adaptive-query error by turn}} \\
\cmidrule{1-4}
Turn bin & $N$ & MAE (Gy) & RMSE (Gy) \\
1--4 & 967 & 0.319 & 0.442 \\
5--8 & 565 & 0.438 & 0.583 \\
9--12 & 158 & 0.327 & 0.454 \\
13--16 & 42 & 0.300 & 0.408 \\
\bottomrule
\end{tabular*}
\caption{\textbf{Surrogate-verifier evaluation.} Adaptive queries are the
full-solve requests of the representative GPT-5.6 Sol campaign, subsequently
evaluated by Gurobi; 33 timed-out attempts have no paired target and are
excluded, leaving 1{,}732 of 1{,}765 requests. The adaptive within-context
Spearman is computed over at most three full solves per context and therefore
takes few distinct values; it indicates ordering agreement only coarsely. The
adaptive RMSE of $0.492$~Gy and the uncertainty percentile $q_{90}=0.4922$~Gy
are unrelated quantities.}
\label{tab:supp_verifier_eval}
\end{table}
