# Supplementary material for: RadOncGym: An Agent-Based Framework for Radiotherapy Dose-Mimicking Optimization
Source: arXiv:2611.33821 source file (2026-11-25)
Supplement: Supplementary file 10 [file supplementary.tex]

\makeatletter
\def\wacvsection{\@startsection {section}{1}{\z@}
   {-10pt plus -2pt minus -2pt}{7pt} {\large\bf\raggedright}}
\def\wacvsubsection{\@startsection {subsection}{2}{\z@}
   {-8pt plus -2pt minus -2pt}{5pt} {\elvbf\raggedright}}
\makeatother

\renewcommand{\_}{\textunderscore\allowbreak}

\renewcommand{\arraystretch}{1.08}

\setlength{\textfloatsep}{7pt plus 1pt minus 2pt}
\setlength{\dbltextfloatsep}{7pt plus 1pt minus 2pt}
\setlength{\floatsep}{7pt plus 1pt minus 2pt}
\setlength{\dblfloatsep}{7pt plus 1pt minus 2pt}
\renewcommand{\topfraction}{0.95}
\renewcommand{\dbltopfraction}{0.95}
\renewcommand{\textfraction}{0.05}
\setcounter{topnumber}{5}
\setcounter{dbltopnumber}{5}

\raggedbottom

\makeatletter
\setlength{\@dblfptop}{0pt}
\setlength{\@dblfpsep}{14pt plus 4pt}
\setlength{\@dblfpbot}{0pt plus 1fil}
\makeatother

\setcounter{table}{0}
\setcounter{figure}{0}
\setcounter{equation}{0}
\renewcommand{\thetable}{S\arabic{table}}
\renewcommand{\thefigure}{S\arabic{figure}}
\renewcommand{\theHtable}{supplement.\arabic{table}}
\renewcommand{\theHfigure}{supplement.\arabic{figure}}
\renewcommand{\theHequation}{supplement.\arabic{equation}}

\maketitlesupplementary
\phantomsection
\pdfbookmark[0]{Supplementary Material}{supplementary-material}

\setcounter{tocdepth}{2}
\addtocontents{toc}{\protect\setcounter{tocdepth}{2}}
{\makeatletter\renewcommand{\numberline}[1]{#1\hspace{1em}}%
\renewcommand{\@pnumwidth}{1.8em}\renewcommand{\@tocrmarg}{2.8em}\makeatother
\tableofcontents}
\clearpage
\appendix

\input{supplement/reproducibility}
\input{supplement/prompts}
\input{supplement/planning_formulation}
\input{supplement/agent_observation}
\input{supplement/surrogate_verifier}
\input{supplement/baselines_and_controls}
\input{supplement/statistical_uncertainty}

\input{supplement/agent_behavior}
\input{supplement/example_episode}
\input{supplement/clinical_safety}
